# Supplementary material for: Faster Deep Reinforcement Learning with Slower Online Network
Source: arXiv:2112.05848 source file (2023-04-17)
Supplement: Supplementary file 1 [file 6_learning_curves_per_appendix.tex]

\begin{figure}
\centering\captionsetup[subfigure]{justification=centering}
\begin{subfigure}[t]{ .18\textwidth} 
\centering 
\includegraphics[width=\textwidth]{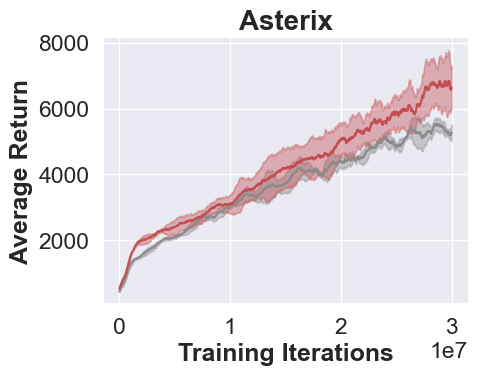} 
\label{fig:6_learning_curves_per_appendix/AsterixNoFrameskip-v0_5_learning_curves_appendix.png} 
\end{subfigure}% 
~ 
\begin{subfigure}[t]{ .18\textwidth} 
\centering 
\includegraphics[width=\textwidth]{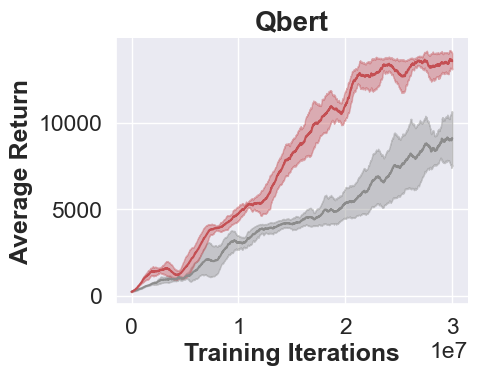} 
\label{fig:6_learning_curves_per_appendix/QbertNoFrameskip-v0_5_learning_curves_appendix.png} 
\end{subfigure}% 
~ 
\begin{subfigure}[t]{ .18\textwidth} 
\centering 
\includegraphics[width=\textwidth]{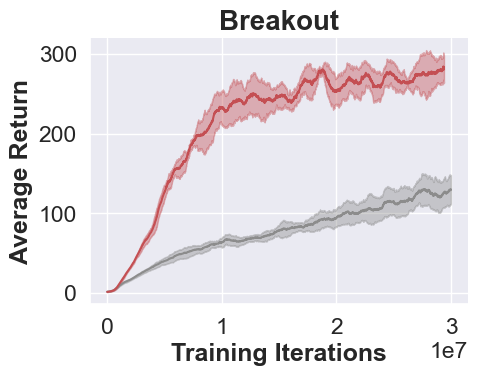} 
\label{fig:6_learning_curves_per_appendix/BreakoutNoFrameskip-v0_5_learning_curves_appendix.png} 
\end{subfigure}% 
~ 
\begin{subfigure}[t]{ .18\textwidth} 
\centering 
\includegraphics[width=\textwidth]{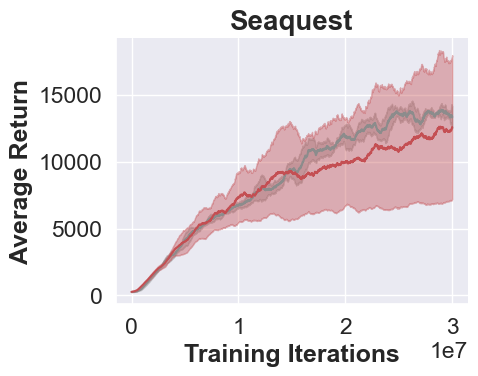} 
\label{fig:6_learning_curves_per_appendix/SeaquestNoFrameskip-v0_5_learning_curves_appendix.png} 
\end{subfigure}% 
~ 
\begin{subfigure}[t]{ .18\textwidth} 
\centering 
\includegraphics[width=\textwidth]{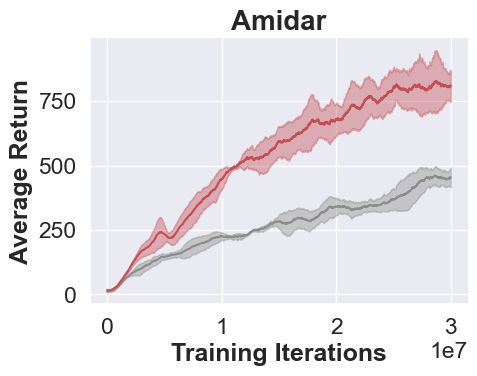} 
\label{fig:6_learning_curves_per_appendix/AmidarNoFrameskip-v0_5_learning_curves_appendix.png} 
\end{subfigure}% 

\begin{subfigure}[t]{ .18\textwidth} 
\centering 
\includegraphics[width=\textwidth]{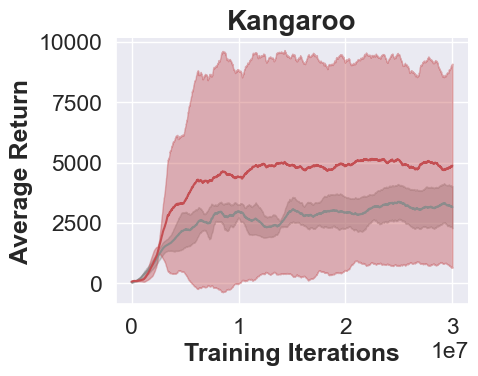} 
\label{fig:6_learning_curves_per_appendix/KangarooNoFrameskip-v0_5_learning_curves_appendix.png} 
\end{subfigure}% 
~ 
\begin{subfigure}[t]{ .18\textwidth} 
\centering 
\includegraphics[width=\textwidth]{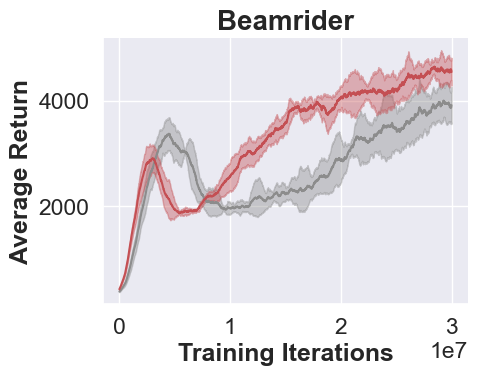} 
\label{fig:6_learning_curves_per_appendix/BeamRiderNoFrameskip-v0_5_learning_curves_appendix.png} 
\end{subfigure}% 
~ 
\begin{subfigure}[t]{ .18\textwidth} 
\centering 
\includegraphics[width=\textwidth]{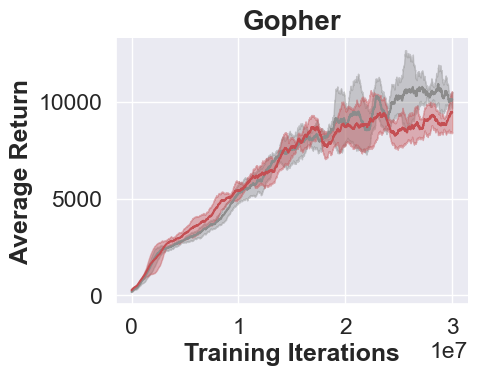} 
\label{fig:6_learning_curves_per_appendix/GopherNoFrameskip-v0_5_learning_curves_appendix.png} 
\end{subfigure}% 
~ 
\begin{subfigure}[t]{ .18\textwidth} 
\centering 
\includegraphics[width=\textwidth]{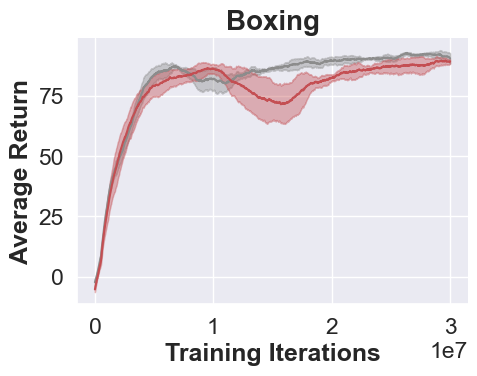} 
\label{fig:6_learning_curves_per_appendix/BoxingNoFrameskip-v0_5_learning_curves_appendix.png} 
\end{subfigure}% 
~ 
\begin{subfigure}[t]{ .18\textwidth} 
\centering 
\includegraphics[width=\textwidth]{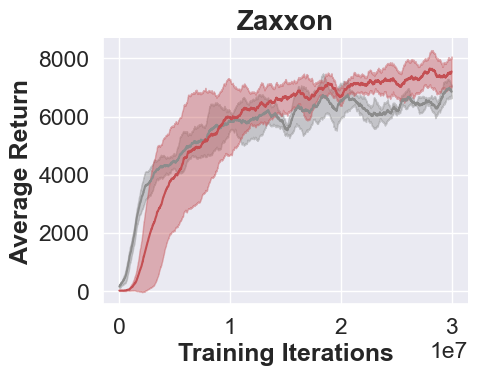} 
\label{fig:6_learning_curves_per_appendix/ZaxxonNoFrameskip-v0_5_learning_curves_appendix.png} 
\end{subfigure}% 

\begin{subfigure}[t]{ .18\textwidth} 
\centering 
\includegraphics[width=\textwidth]{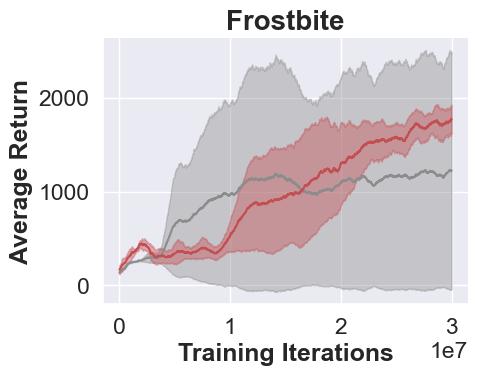} 
\label{fig:6_learning_curves_per_appendix/FrostbiteNoFrameskip-v0_5_learning_curves_appendix.png} 
\end{subfigure}% 
~ 
\begin{subfigure}[t]{ .18\textwidth} 
\centering 
\includegraphics[width=\textwidth]{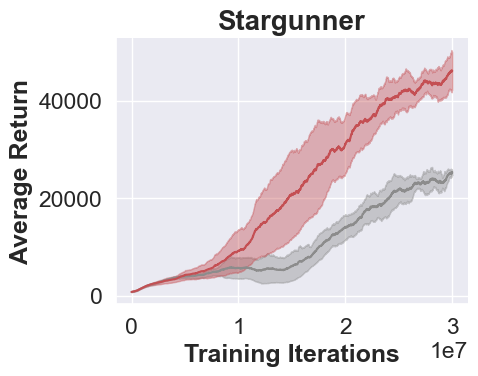} 
\label{fig:6_learning_curves_per_appendix/StarGunnerNoFrameskip-v0_5_learning_curves_appendix.png} 
\end{subfigure}% 
~ 
\begin{subfigure}[t]{ .18\textwidth} 
\centering 
\includegraphics[width=\textwidth]{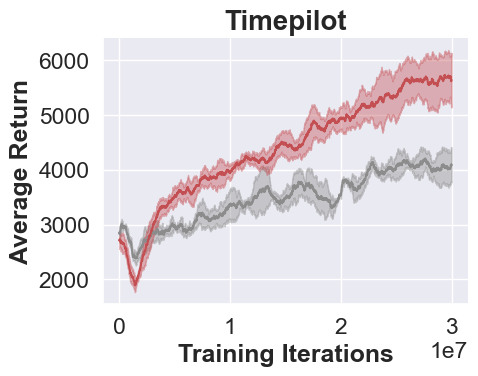} 
\label{fig:6_learning_curves_per_appendix/TimePilotNoFrameskip-v0_5_learning_curves_appendix.png} 
\end{subfigure}% 
~ 
\begin{subfigure}[t]{ .18\textwidth} 
\centering 
\includegraphics[width=\textwidth]{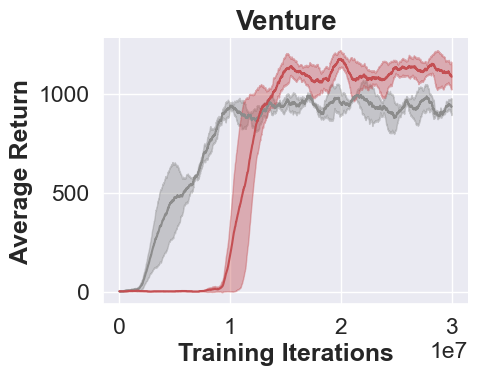} 
\label{fig:6_learning_curves_per_appendix/VentureNoFrameskip-v0_5_learning_curves_appendix.png} 
\end{subfigure}% 
~ 
\begin{subfigure}[t]{ .18\textwidth} 
\centering 
\includegraphics[width=\textwidth]{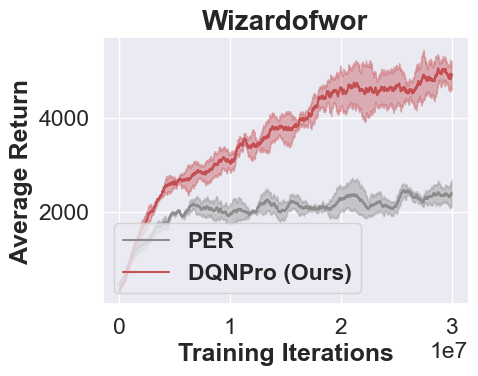} 
\label{fig:6_learning_curves_per_appendix/WizardOfWorNoFrameskip-v0_5_learning_curves_appendix.png} 
\end{subfigure}% 

\caption{
\textbf{Learning curves for DQN with prioritized experience replay (PER) (gary) and \algname{} (red)} on 15 Atari games. X-axis indicates the number of steps from the environment used in training and Y-axis shows average undiscounted return.
%A comparison between DQNPro and Prioritized Experience Replay (PER) citation zzz.
} 
\label{fig:main-per} 
\end{figure}
