# Supplementary material for: Faster Deep Reinforcement Learning with Slower Online Network
Source: arXiv:2112.05848 source file (2023-04-17)
Supplement: Supplementary file 2 [file 7_learning_curves_polyak_appendix.tex]

\begin{figure}
\centering\captionsetup[subfigure]{justification=centering}
\begin{subfigure}[t]{ 0.2\textwidth} 
\centering 
\includegraphics[width=\textwidth]{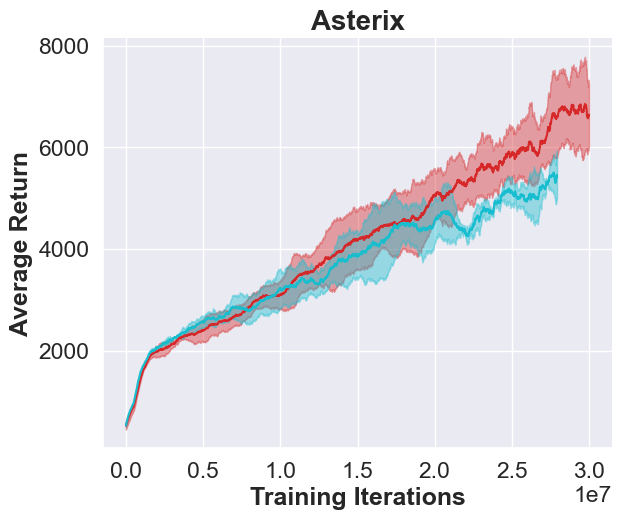} 
\label{fig:7_learning_curves_polyak_appendix/AsterixNoFrameskip-v0_7_learning_curves_polyak_appendix.png} 
\end{subfigure}% 
~ 
\begin{subfigure}[t]{ 0.2\textwidth} 
\centering 
\includegraphics[width=\textwidth]{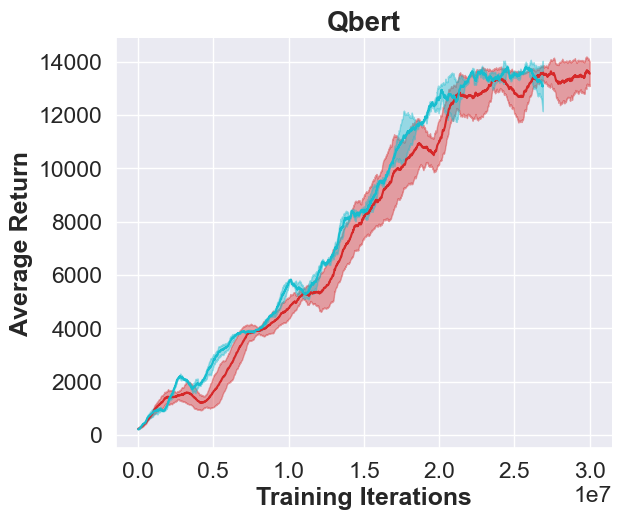} 
\label{fig:7_learning_curves_polyak_appendix/QbertNoFrameskip-v0_7_learning_curves_polyak_appendix.png} 
\end{subfigure}% 
~ 
\begin{subfigure}[t]{ 0.2\textwidth} 
\centering 
\includegraphics[width=\textwidth]{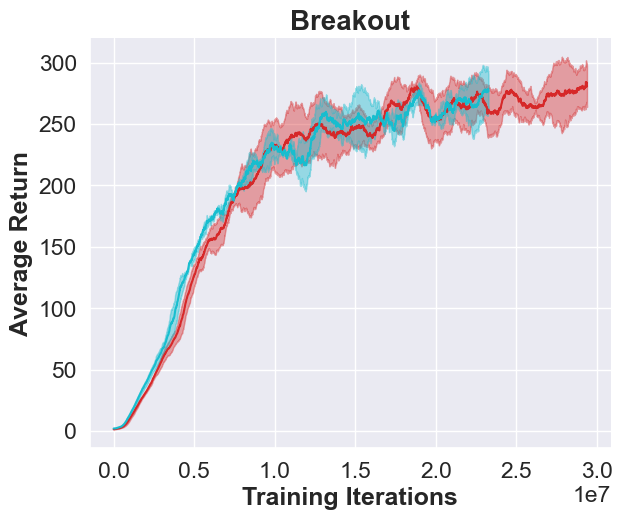} 
\label{fig:7_learning_curves_polyak_appendix/BreakoutNoFrameskip-v0_7_learning_curves_polyak_appendix.png} 
\end{subfigure}% 
~ 
\begin{subfigure}[t]{ 0.2\textwidth} 
\centering 
\includegraphics[width=\textwidth]{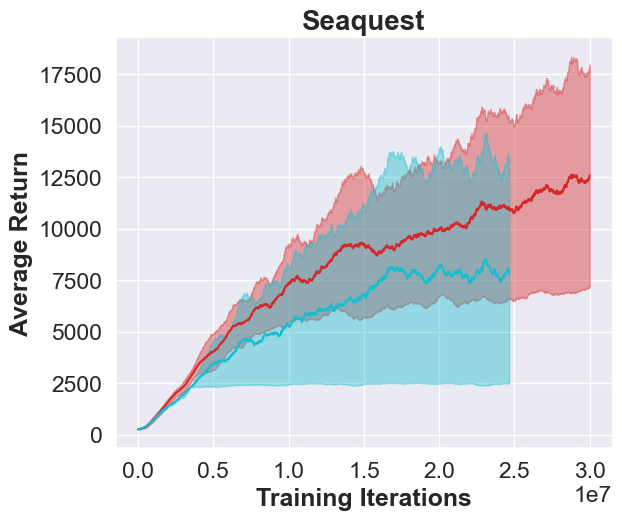} 
\label{fig:7_learning_curves_polyak_appendix/SeaquestNoFrameskip-v0_7_learning_curves_polyak_appendix.png} 
\end{subfigure}% 
~ 
\begin{subfigure}[t]{ 0.2\textwidth} 
\centering 
\includegraphics[width=\textwidth]{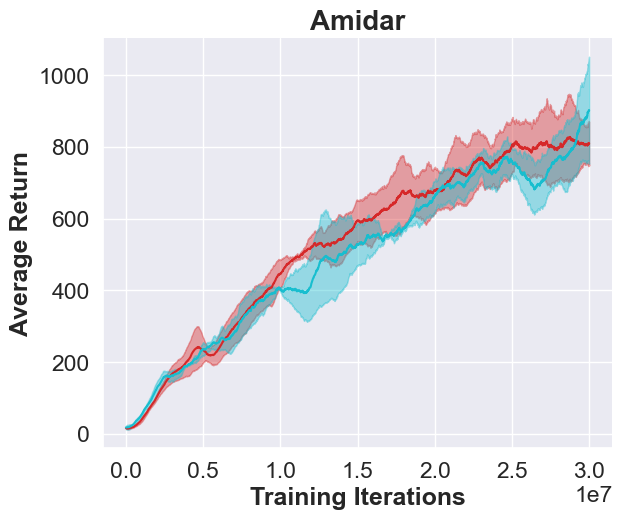} 
\label{fig:7_learning_curves_polyak_appendix/AmidarNoFrameskip-v0_7_learning_curves_polyak_appendix.png} 
\end{subfigure}% 

\begin{subfigure}[t]{ 0.2\textwidth} 
\centering 
\includegraphics[width=\textwidth]{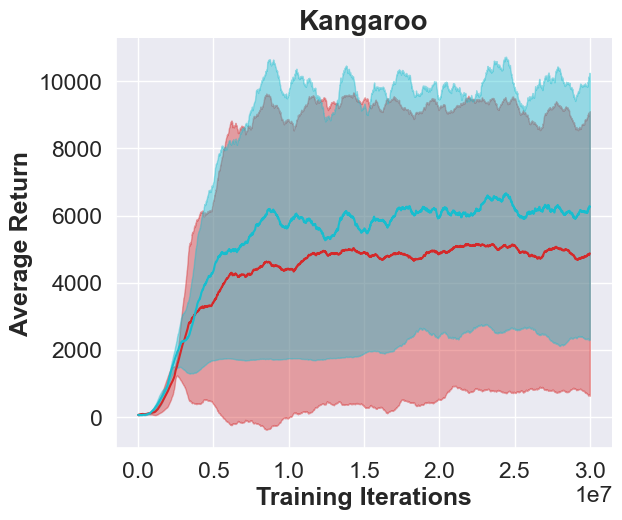} 
\label{fig:7_learning_curves_polyak_appendix/KangarooNoFrameskip-v0_7_learning_curves_polyak_appendix.png} 
\end{subfigure}% 
~ 
\begin{subfigure}[t]{ 0.2\textwidth} 
\centering 
\includegraphics[width=\textwidth]{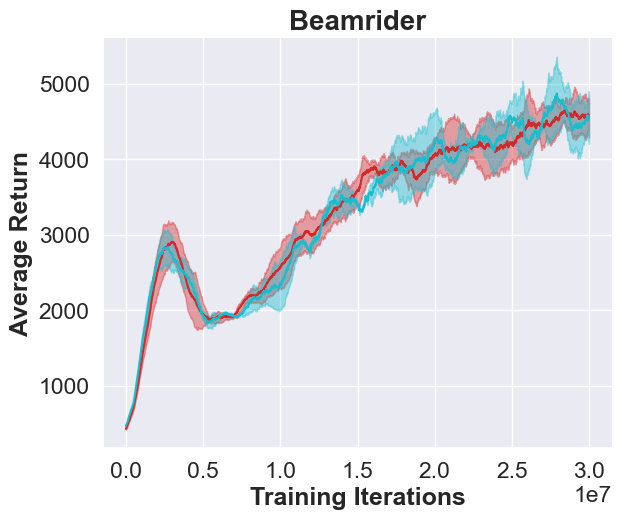} 
\label{fig:7_learning_curves_polyak_appendix/BeamRiderNoFrameskip-v0_7_learning_curves_polyak_appendix.png} 
\end{subfigure}% 
~ 
\begin{subfigure}[t]{ 0.2\textwidth} 
\centering 
\includegraphics[width=\textwidth]{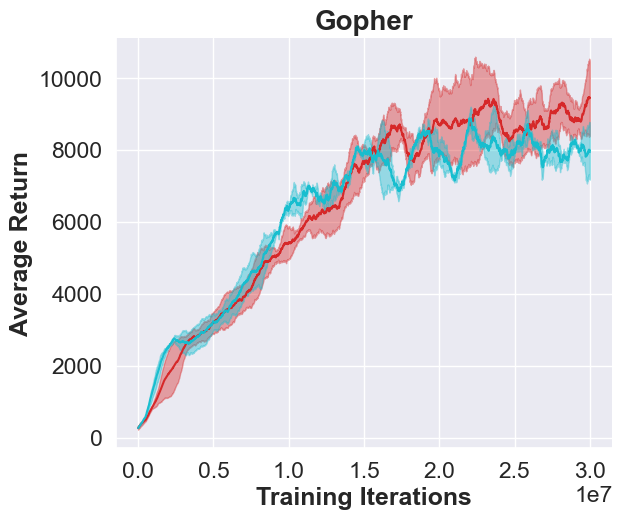} 
\label{fig:7_learning_curves_polyak_appendix/GopherNoFrameskip-v0_7_learning_curves_polyak_appendix.png} 
\end{subfigure}% 
~ 
\begin{subfigure}[t]{ 0.2\textwidth} 
\centering 
\includegraphics[width=\textwidth]{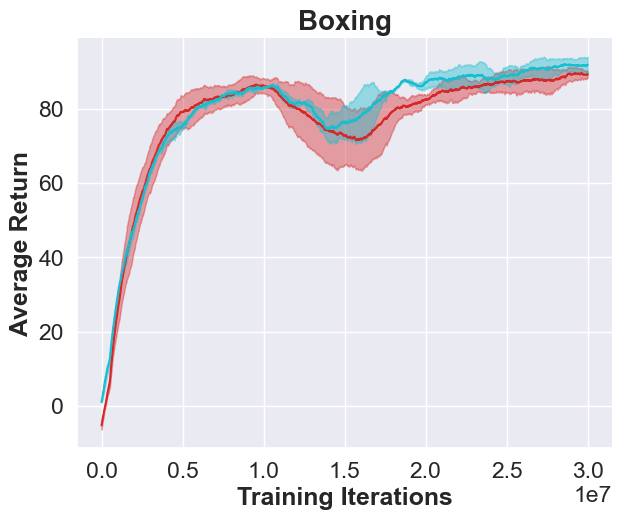} 
\label{fig:7_learning_curves_polyak_appendix/BoxingNoFrameskip-v0_7_learning_curves_polyak_appendix.png} 
\end{subfigure}% 
~ 
\begin{subfigure}[t]{ 0.2\textwidth} 
\centering 
\includegraphics[width=\textwidth]{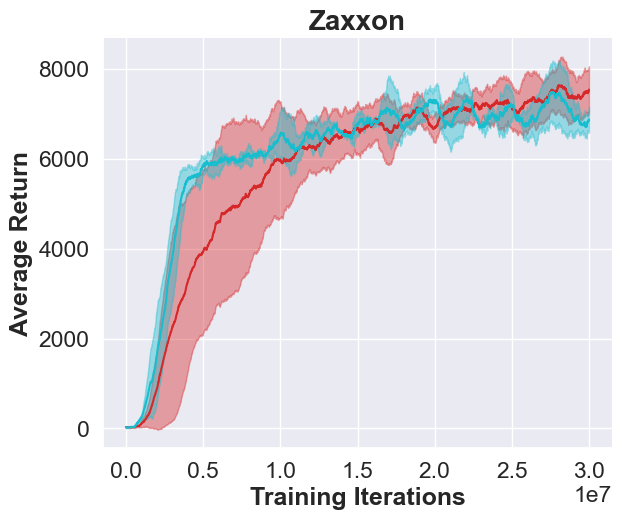} 
\label{fig:7_learning_curves_polyak_appendix/ZaxxonNoFrameskip-v0_7_learning_curves_polyak_appendix.png} 
\end{subfigure}% 

\begin{subfigure}[t]{ 0.2\textwidth} 
\centering 
\includegraphics[width=\textwidth]{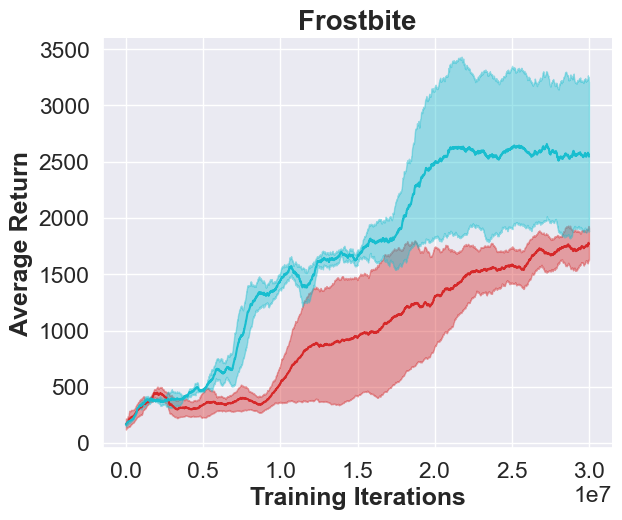} 
\label{fig:7_learning_curves_polyak_appendix/FrostbiteNoFrameskip-v0_7_learning_curves_polyak_appendix.png} 
\end{subfigure}% 
~ 
\begin{subfigure}[t]{ 0.2\textwidth} 
\centering 
\includegraphics[width=\textwidth]{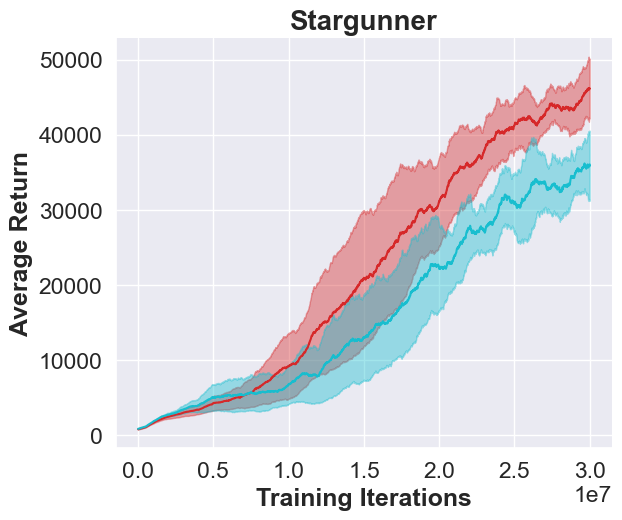} 
\label{fig:7_learning_curves_polyak_appendix/StarGunnerNoFrameskip-v0_7_learning_curves_polyak_appendix.png} 
\end{subfigure}% 
~ 
\begin{subfigure}[t]{ 0.2\textwidth} 
\centering 
\includegraphics[width=\textwidth]{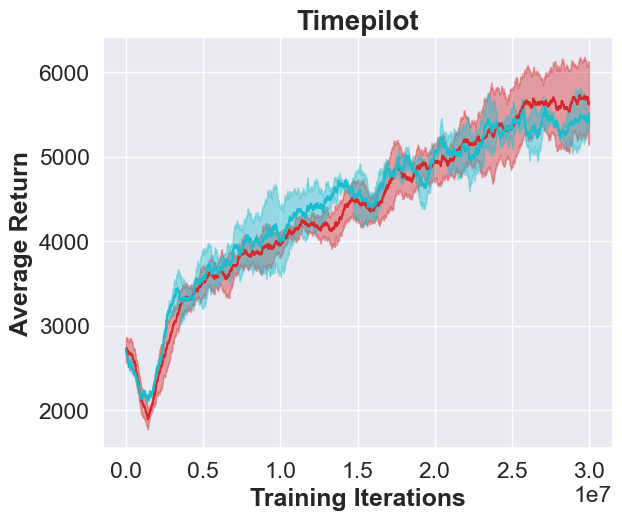} 
\label{fig:7_learning_curves_polyak_appendix/TimePilotNoFrameskip-v0_7_learning_curves_polyak_appendix.png} 
\end{subfigure}% 
~ 
\begin{subfigure}[t]{ 0.2\textwidth} 
\centering 
\includegraphics[width=\textwidth]{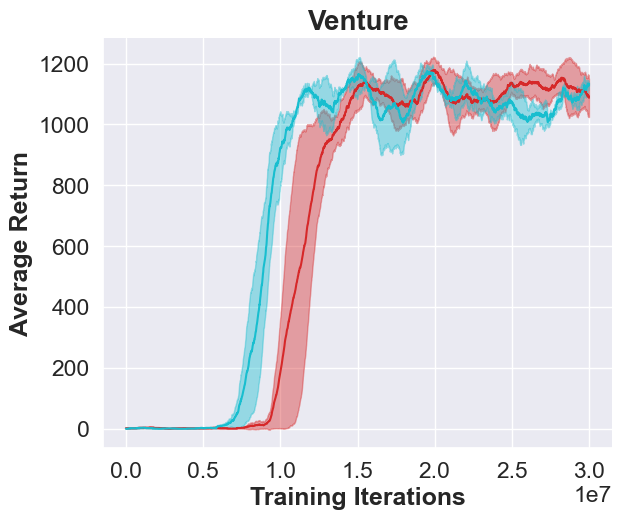} 
\label{fig:7_learning_curves_polyak_appendix/VentureNoFrameskip-v0_7_learning_curves_polyak_appendix.png} 
\end{subfigure}% 
~ 
\begin{subfigure}[t]{ 0.2\textwidth} 
\centering 
\includegraphics[width=\textwidth]{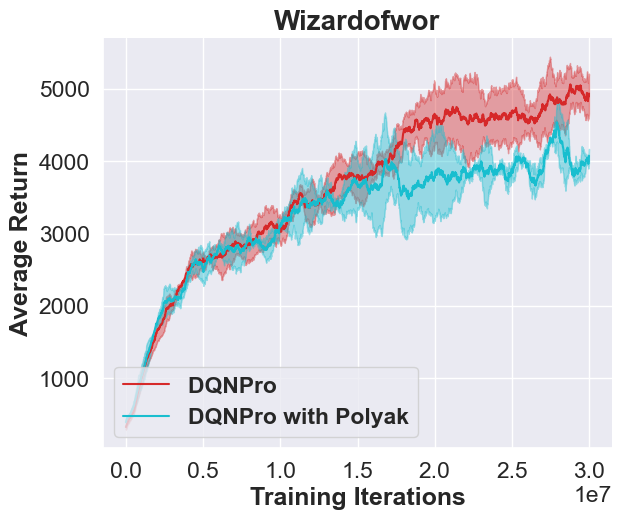} 
\label{fig:7_learning_curves_polyak_appendix/WizardOfWorNoFrameskip-v0_7_learning_curves_polyak_appendix.png} 
\end{subfigure}% 

\caption{\textbf{A comparison between DQNPro and DQNPro with Polyak updating}.} 
\label{fig:main-poly} 
\end{figure}
