# Supplementary material for: Faster Deep Reinforcement Learning with Slower Online Network
Source: arXiv:2112.05848 source file (2023-04-17)
Supplement: Supplementary file 4 [file 5_learning_curves_appendix.tex]

\begin{figure}
\centering\captionsetup[subfigure]{justification=centering}
\begin{subfigure}[t]{ .18\textwidth} 
\centering 
\includegraphics[width=\textwidth]{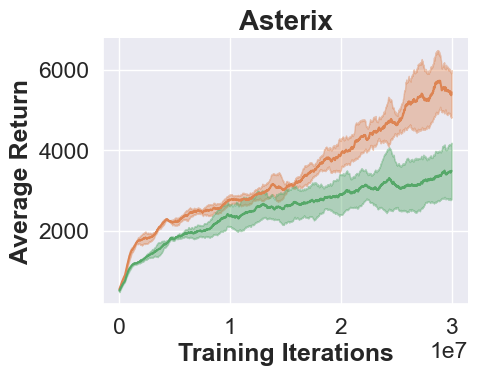} 
\label{fig:5_learning_curves_appendix/AsterixNoFrameskip-v0_5_learning_curves_appendix.png} 
\end{subfigure}% 
~ 
\begin{subfigure}[t]{ .18\textwidth} 
\centering 
\includegraphics[width=\textwidth]{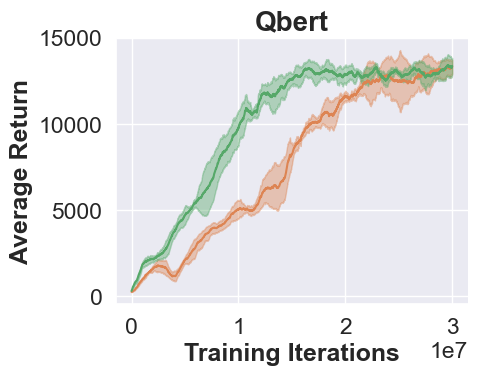} 
\label{fig:5_learning_curves_appendix/QbertNoFrameskip-v0_5_learning_curves_appendix.png} 
\end{subfigure}% 
~ 
\begin{subfigure}[t]{ .18\textwidth} 
\centering 
\includegraphics[width=\textwidth]{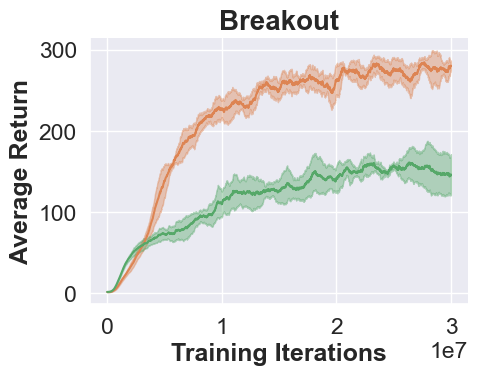} 
\label{fig:5_learning_curves_appendix/BreakoutNoFrameskip-v0_5_learning_curves_appendix.png} 
\end{subfigure}% 
~ 
\begin{subfigure}[t]{ .18\textwidth} 
\centering 
\includegraphics[width=\textwidth]{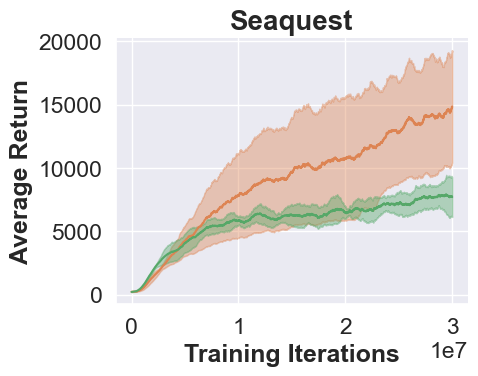} 
\label{fig:5_learning_curves_appendix/SeaquestNoFrameskip-v0_5_learning_curves_appendix.png} 
\end{subfigure}% 
~ 
\begin{subfigure}[t]{ .18\textwidth} 
\centering 
\includegraphics[width=\textwidth]{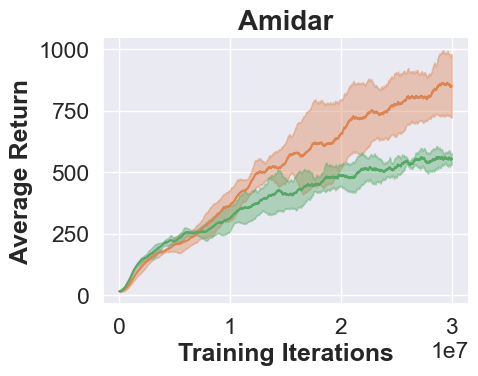} 
\label{fig:5_learning_curves_appendix/AmidarNoFrameskip-v0_5_learning_curves_appendix.png} 
\end{subfigure}% 

\begin{subfigure}[t]{ .18\textwidth} 
\centering 
\includegraphics[width=\textwidth]{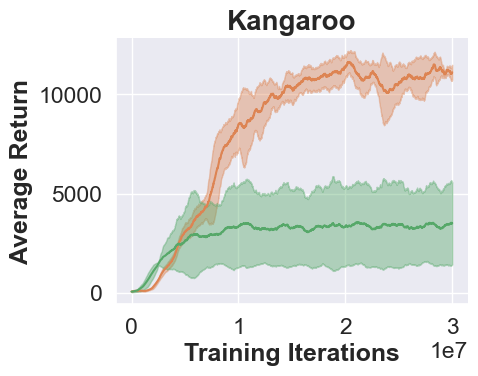} 
\label{fig:5_learning_curves_appendix/KangarooNoFrameskip-v0_5_learning_curves_appendix.png} 
\end{subfigure}% 
~ 
\begin{subfigure}[t]{ .18\textwidth} 
\centering 
\includegraphics[width=\textwidth]{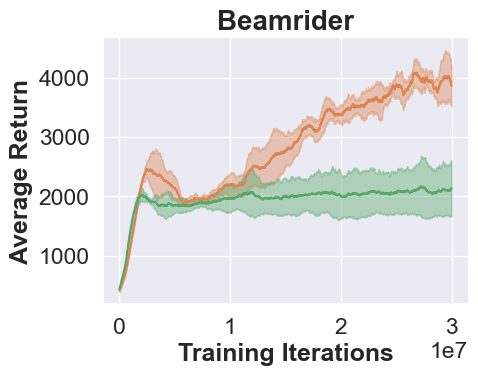} 
\label{fig:5_learning_curves_appendix/BeamRiderNoFrameskip-v0_5_learning_curves_appendix.png} 
\end{subfigure}% 
~ 
\begin{subfigure}[t]{ .18\textwidth} 
\centering 
\includegraphics[width=\textwidth]{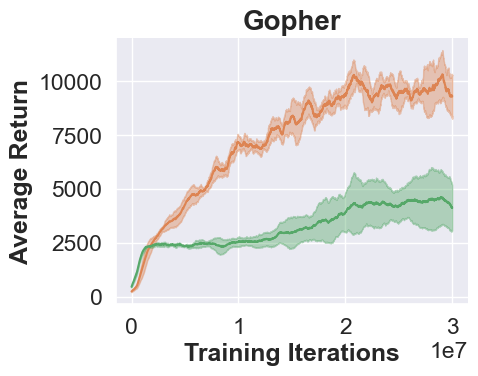} 
\label{fig:5_learning_curves_appendix/GopherNoFrameskip-v0_5_learning_curves_appendix.png} 
\end{subfigure}% 
~ 
\begin{subfigure}[t]{ .18\textwidth} 
\centering 
\includegraphics[width=\textwidth]{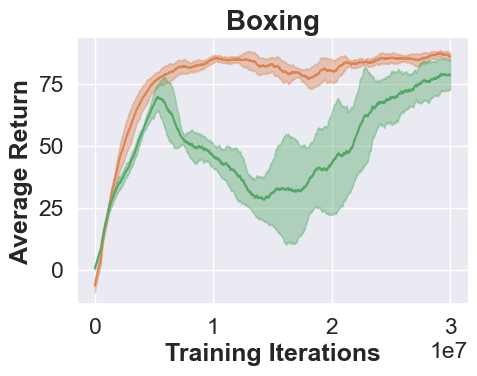} 
\label{fig:5_learning_curves_appendix/BoxingNoFrameskip-v0_5_learning_curves_appendix.png} 
\end{subfigure}% 
~ 
\begin{subfigure}[t]{ .18\textwidth} 
\centering 
\includegraphics[width=\textwidth]{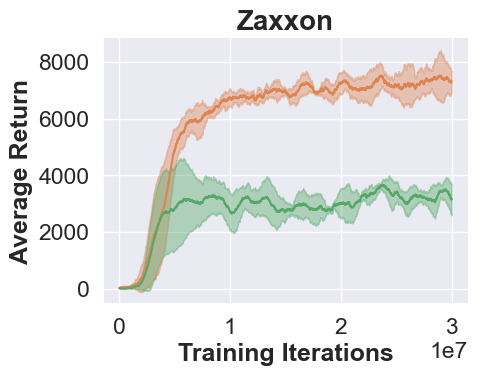} 
\label{fig:5_learning_curves_appendix/ZaxxonNoFrameskip-v0_5_learning_curves_appendix.png} 
\end{subfigure}% 

\begin{subfigure}[t]{ .18\textwidth} 
\centering 
\includegraphics[width=\textwidth]{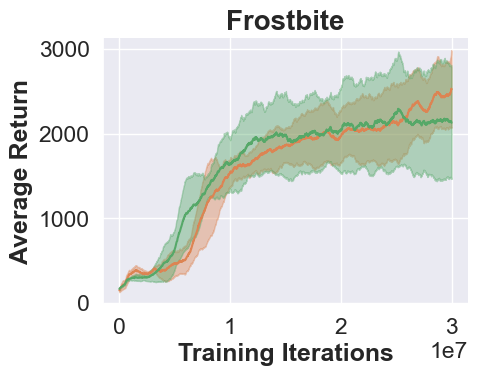} 
\label{fig:5_learning_curves_appendix/FrostbiteNoFrameskip-v0_5_learning_curves_appendix.png} 
\end{subfigure}% 
~ 
\begin{subfigure}[t]{ .18\textwidth} 
\centering 
\includegraphics[width=\textwidth]{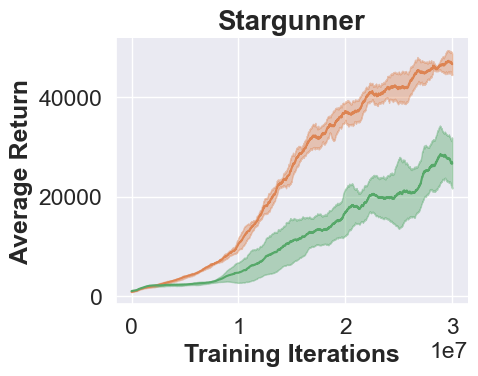} 
\label{fig:5_learning_curves_appendix/StarGunnerNoFrameskip-v0_5_learning_curves_appendix.png} 
\end{subfigure}% 
~ 
\begin{subfigure}[t]{ .18\textwidth} 
\centering 
\includegraphics[width=\textwidth]{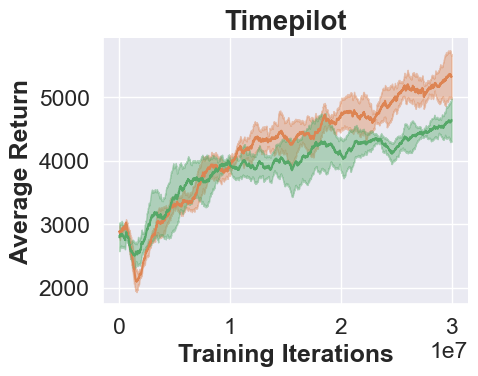} 
\label{fig:5_learning_curves_appendix/TimePilotNoFrameskip-v0_5_learning_curves_appendix.png} 
\end{subfigure}% 
~ 
\begin{subfigure}[t]{ .18\textwidth} 
\centering 
\includegraphics[width=\textwidth]{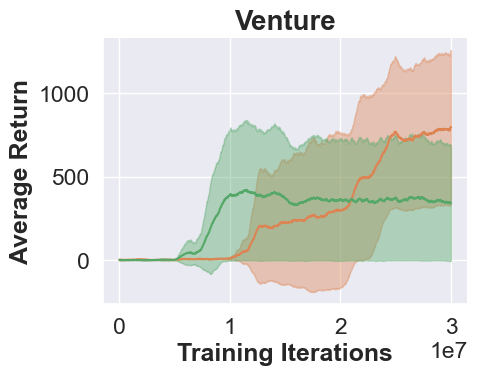} 
\label{fig:5_learning_curves_appendix/VentureNoFrameskip-v0_5_learning_curves_appendix.png} 
\end{subfigure}% 
~ 
\begin{subfigure}[t]{ .18\textwidth} 
\centering 
\includegraphics[width=\textwidth]{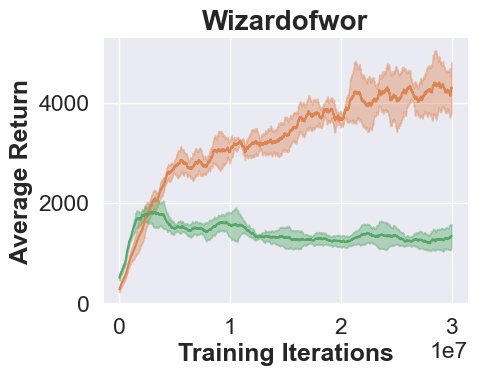} 
\label{fig:5_learning_curves_appendix/WizardOfWorNoFrameskip-v0_5_learning_curves_appendix.png} 
\end{subfigure}% 

\begin{subfigure}[t]{ .18\textwidth} 
\centering 
\includegraphics[width=\textwidth]{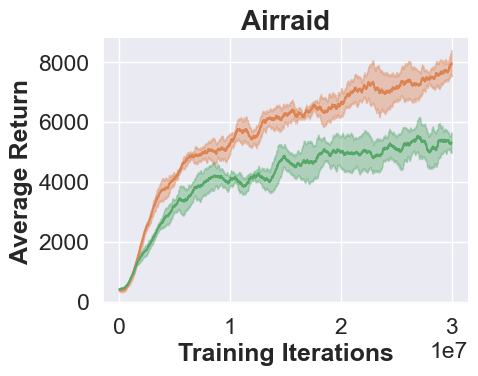} 
\label{fig:5_learning_curves_appendix/AirRaidNoFrameskip-v0_5_learning_curves_appendix.png} 
\end{subfigure}% 
~ 
\begin{subfigure}[t]{ .18\textwidth} 
\centering 
\includegraphics[width=\textwidth]{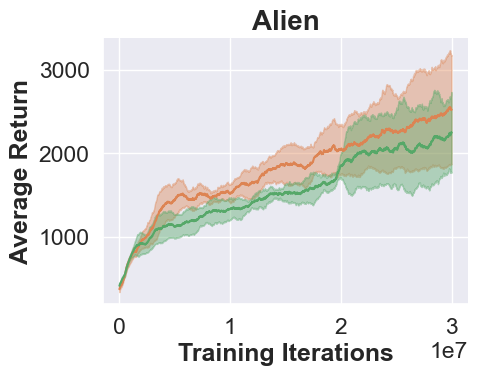} 
\label{fig:5_learning_curves_appendix/AlienNoFrameskip-v0_5_learning_curves_appendix.png} 
\end{subfigure}% 
~ 
\begin{subfigure}[t]{ .18\textwidth} 
\centering 
\includegraphics[width=\textwidth]{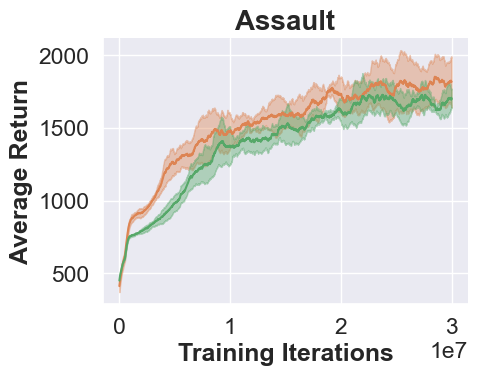} 
\label{fig:5_learning_curves_appendix/AssaultNoFrameskip-v0_5_learning_curves_appendix.png} 
\end{subfigure}% 
~ 
\begin{subfigure}[t]{ .18\textwidth} 
\centering 
\includegraphics[width=\textwidth]{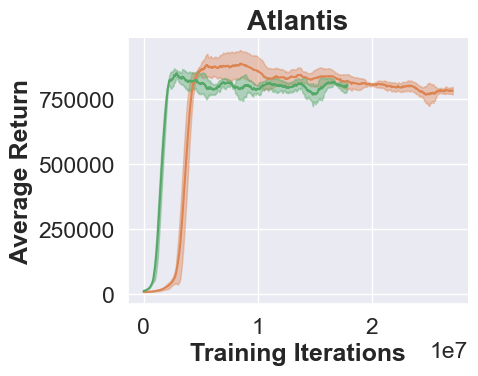} 
\label{fig:5_learning_curves_appendix/AtlantisNoFrameskip-v0_5_learning_curves_appendix.png} 
\end{subfigure}% 
~ 
\begin{subfigure}[t]{ .18\textwidth} 
\centering 
\includegraphics[width=\textwidth]{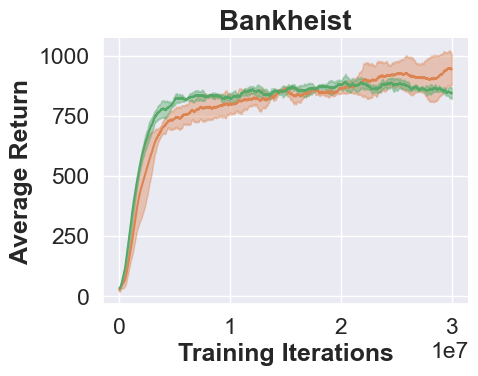} 
\label{fig:5_learning_curves_appendix/BankHeistNoFrameskip-v0_5_learning_curves_appendix.png} 
\end{subfigure}% 

\begin{subfigure}[t]{ .18\textwidth} 
\centering 
\includegraphics[width=\textwidth]{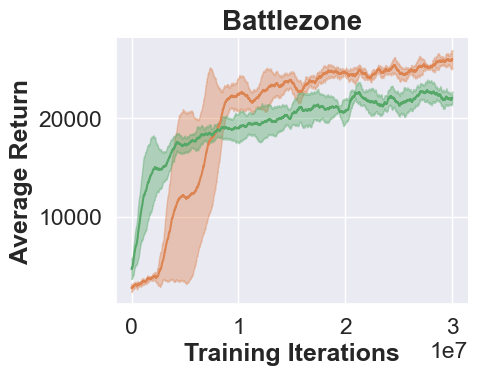} 
\label{fig:5_learning_curves_appendix/BattleZoneNoFrameskip-v0_5_learning_curves_appendix.png} 
\end{subfigure}% 
~ 
\begin{subfigure}[t]{ .18\textwidth} 
\centering 
\includegraphics[width=\textwidth]{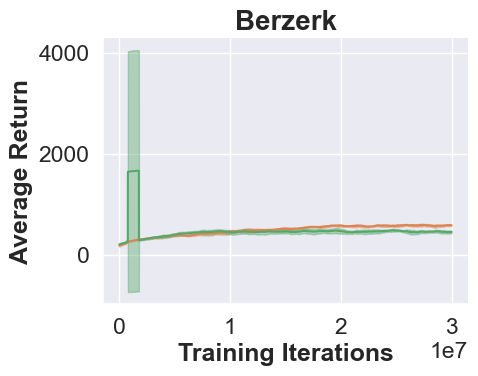} 
\label{fig:5_learning_curves_appendix/BerzerkNoFrameskip-v0_5_learning_curves_appendix.png} 
\end{subfigure}% 
~ 
\begin{subfigure}[t]{ .18\textwidth} 
\centering 
\includegraphics[width=\textwidth]{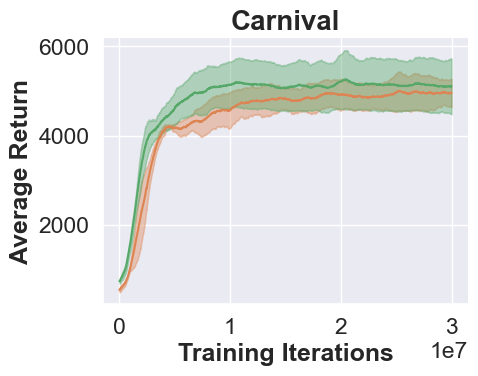} 
\label{fig:5_learning_curves_appendix/CarnivalNoFrameskip-v0_5_learning_curves_appendix.png} 
\end{subfigure}% 
~ 
\begin{subfigure}[t]{ .18\textwidth} 
\centering 
\includegraphics[width=\textwidth]{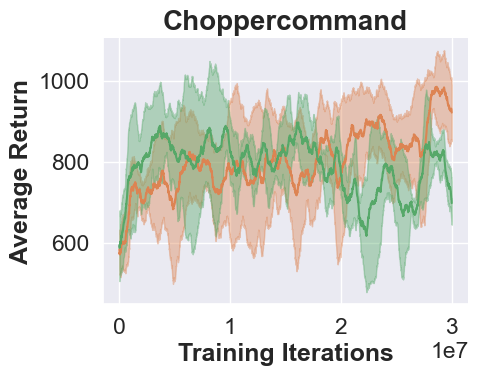} 
\label{fig:5_learning_curves_appendix/ChopperCommandNoFrameskip-v0_5_learning_curves_appendix.png} 
\end{subfigure}% 
~ 
\begin{subfigure}[t]{ .18\textwidth} 
\centering 
\includegraphics[width=\textwidth]{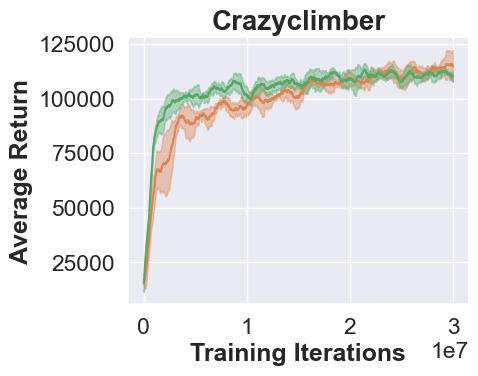} 
\label{fig:5_learning_curves_appendix/CrazyClimberNoFrameskip-v0_5_learning_curves_appendix.png} 
\end{subfigure}% 

\begin{subfigure}[t]{ .18\textwidth} 
\centering 
\includegraphics[width=\textwidth]{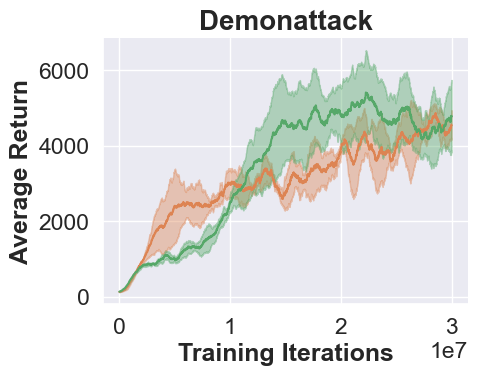} 
\label{fig:5_learning_curves_appendix/DemonAttackNoFrameskip-v0_5_learning_curves_appendix.png} 
\end{subfigure}% 
~ 
\begin{subfigure}[t]{ .18\textwidth} 
\centering 
\includegraphics[width=\textwidth]{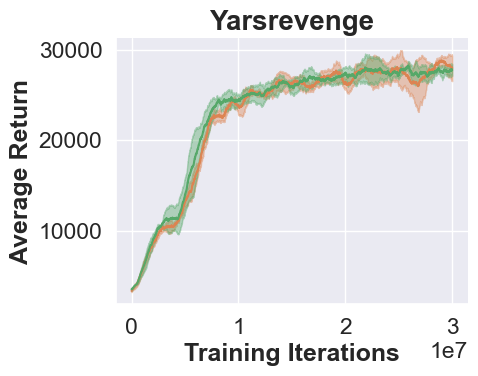} 
\label{fig:5_learning_curves_appendix/YarsRevengeNoFrameskip-v0_5_learning_curves_appendix.png} 
\end{subfigure}% 
~ 
\begin{subfigure}[t]{ .18\textwidth} 
\centering 
\includegraphics[width=\textwidth]{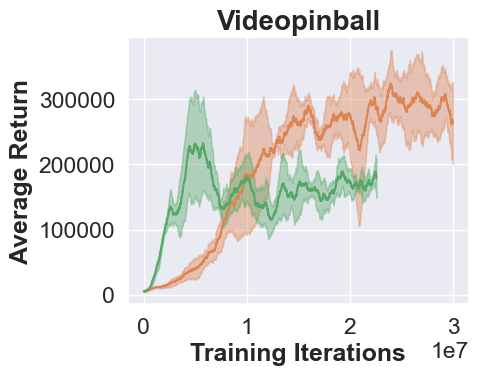} 
\label{fig:5_learning_curves_appendix/VideoPinballNoFrameskip-v0_5_learning_curves_appendix.png} 
\end{subfigure}% 
~ 
\begin{subfigure}[t]{ .18\textwidth} 
\centering 
\includegraphics[width=\textwidth]{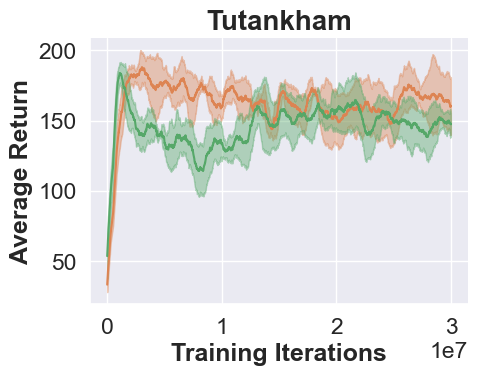} 
\label{fig:5_learning_curves_appendix/TutankhamNoFrameskip-v0_5_learning_curves_appendix.png} 
\end{subfigure}% 
~ 
\begin{subfigure}[t]{ .18\textwidth} 
\centering 
\includegraphics[width=\textwidth]{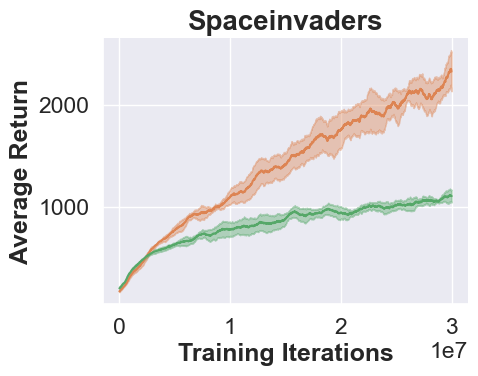} 
\label{fig:5_learning_curves_appendix/SpaceInvadersNoFrameskip-v0_5_learning_curves_appendix.png} 
\end{subfigure}% 

\begin{subfigure}[t]{ .18\textwidth} 
\centering 
\includegraphics[width=\textwidth]{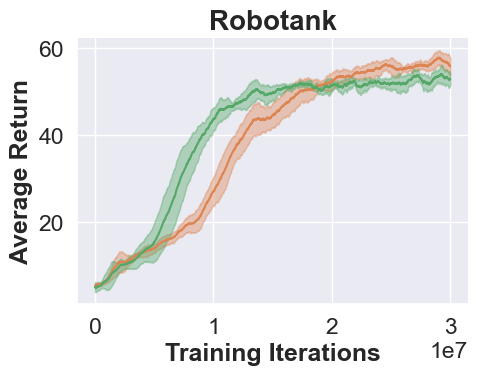} 
\label{fig:5_learning_curves_appendix/RobotankNoFrameskip-v0_5_learning_curves_appendix.png} 
\end{subfigure}% 
~ 
\begin{subfigure}[t]{ .18\textwidth} 
\centering 
\includegraphics[width=\textwidth]{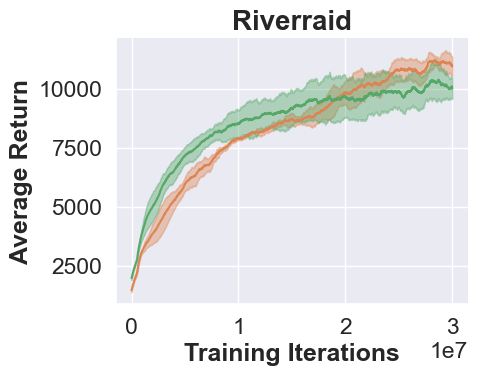} 
\label{fig:5_learning_curves_appendix/RiverraidNoFrameskip-v0_5_learning_curves_appendix.png} 
\end{subfigure}% 
~ 
\begin{subfigure}[t]{ .18\textwidth} 
\centering 
\includegraphics[width=\textwidth]{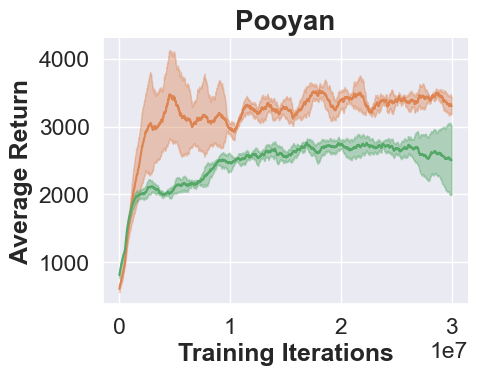} 
\label{fig:5_learning_curves_appendix/PooyanNoFrameskip-v0_5_learning_curves_appendix.png} 
\end{subfigure}% 
~ 
\begin{subfigure}[t]{ .18\textwidth} 
\centering 
\includegraphics[width=\textwidth]{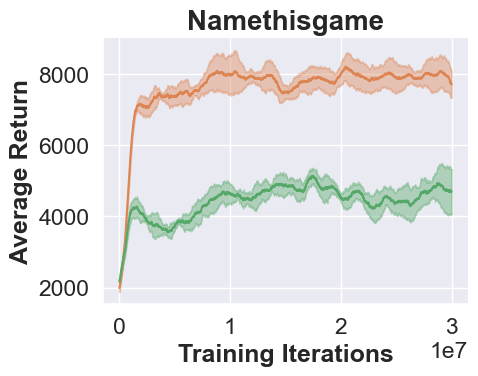} 
\label{fig:5_learning_curves_appendix/NameThisGameNoFrameskip-v0_5_learning_curves_appendix.png} 
\end{subfigure}% 
~ 
\begin{subfigure}[t]{ .18\textwidth} 
\centering 
\includegraphics[width=\textwidth]{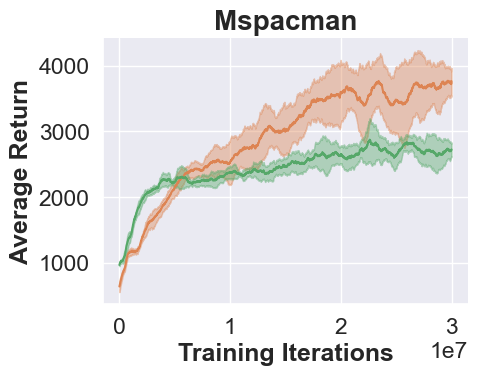} 
\label{fig:5_learning_curves_appendix/MsPacmanNoFrameskip-v0_5_learning_curves_appendix.png} 
\end{subfigure}% 

\begin{subfigure}[t]{ .18\textwidth} 
\centering 
\includegraphics[width=\textwidth]{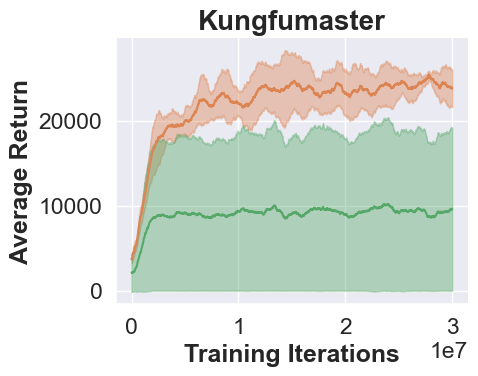} 
\label{fig:5_learning_curves_appendix/KungFuMasterNoFrameskip-v0_5_learning_curves_appendix.png} 
\end{subfigure}% 
~ 
\begin{subfigure}[t]{ .18\textwidth} 
\centering 
\includegraphics[width=\textwidth]{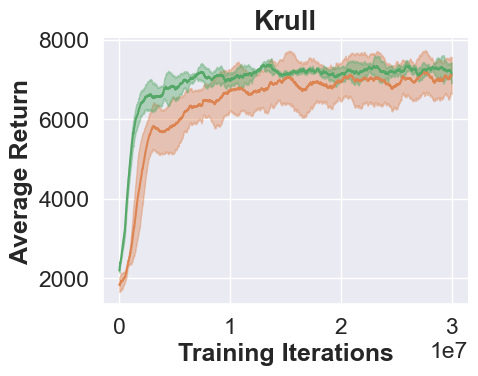} 
\label{fig:5_learning_curves_appendix/KrullNoFrameskip-v0_5_learning_curves_appendix.png} 
\end{subfigure}% 
~ 
\begin{subfigure}[t]{ .18\textwidth} 
\centering 
\includegraphics[width=\textwidth]{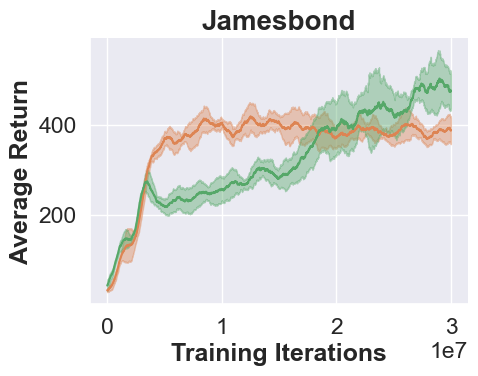} 
\label{fig:5_learning_curves_appendix/JamesbondNoFrameskip-v0_5_learning_curves_appendix.png} 
\end{subfigure}% 
~ 
\begin{subfigure}[t]{ .18\textwidth} 
\centering 
\includegraphics[width=\textwidth]{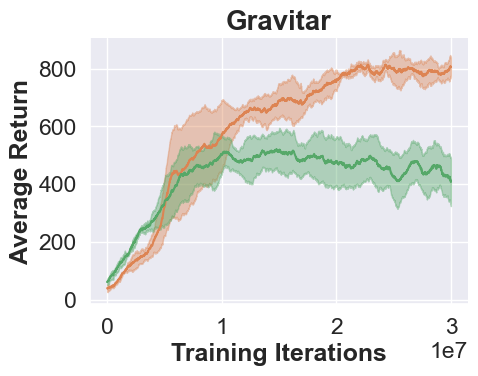} 
\label{fig:5_learning_curves_appendix/GravitarNoFrameskip-v0_5_learning_curves_appendix.png} 
\end{subfigure}% 
~ 
\begin{subfigure}[t]{ .18\textwidth} 
\centering 
\includegraphics[width=\textwidth]{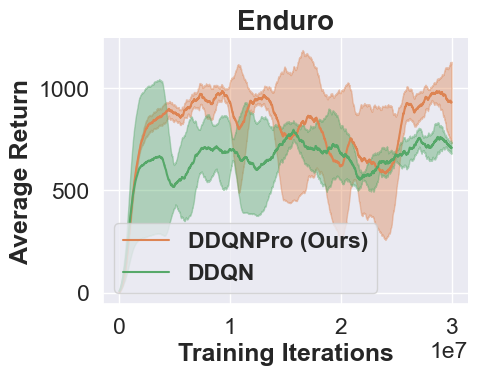} 
\label{fig:5_learning_curves_appendix/EnduroNoFrameskip-v0_5_learning_curves_appendix.png} 
\end{subfigure}% 

\caption{\textbf{Learning curves for DDQN (green) and D\algname{} (orange)} on 40 Atari games. X-axis indicates the number of steps from the environment used in training and Y-axis shows average undiscounted return.}
%A comparison between DDQNPro and DDQN in terms of asymptotic performance.
 
\label{fig:main_ddqn} 
\end{figure}
