# Supplementary material for: Faster Deep Reinforcement Learning with Slower Online Network
Source: arXiv:2112.05848 source file (2023-04-17)
Supplement: Supplementary file 10 [file supplement.tex]

\beginsupplement
\onecolumn
\appendix
\begin{center}
{\LARGE  \bf Appendix: \ 
 \algfullname
}
\end{center}

\section{Implementation Details}\label{sec:app:hyperparams}
\tabref{tab:table-exp-hypers} and \tabref{tab:table-compute-hypers} show hyper-parameters, computing infrastructure, and libraries used for the experiments in this paper for all games tested. Our training and evaluation protocols and the hyper-parameter settings closely follow those of the Dopamine\footnote{\url{https://github.com/google/dopamine}}~\citep{dopamine} baseline. To report performance results, we measured the undiscounted sum of rewards obtained by the learned policy during evaluation. 
\begin{table*}[h!]
    \centering
    \begin{tabular}{|l|c|}
        \hline
        % Shared Hyperparameters & \\ \hline
        \multicolumn{2}{|c|}{\textbf{DQN and DDQN hyper-parameters (shared)}} \\ \hline
        Replay Buffer size & $200000$ \\
        Target update period & $8000$ \\
        Max steps per episode & $27000$ \\
        Evaluation  frequency & $10000$ \\
        Batch Size & $64$ \\
        Update period & $4$ \\
        Number of frame skip & $4$ \\
        Number of episodes to evaluate & $2$ \\
        Update horizon & $1$ \\
        $\epsilon$-greedy (training time)  & $0.01$ \\
        $\epsilon$-greedy (evaluation time)  & $0.001$ \\
        $\epsilon$-greedy decay period  & $250000$ \\
        Burn-in period / Min replay size & $20000$ \\
        Learning rate & $10^{-4}$ \\
        Discount factor ($\gamma$) & $0.99$ \\
        Total number of iterations & $3 \times 10^{7}$  \\
        Sticky actions & True \\
        Optimizer & Adam~\citepsi{KingmaB14}\\
        Network Architecture & Nature DQN network~\citepsi{mnih2015human} \\
        Random Seeds & $\{0,1,2,3\}$
       \\ \hline
        \multicolumn{2}{|c|}{\textbf{Our \algname{} and D\algname{} hyper-parameter}} \\ \hline
        $\color{color_alg} c$ & $\color{color_alg} 0.2$ \\
        \hline
   \end{tabular}
    \caption{\textbf{Hyper-parameters used for all methods for all 40 games of Atari-2600 benchmarks}. All results reported in our paper are averages over repeated runs initialized with each of the random seeds listed above and run for the listed number of episodes.
    }
    \label{tab:table-exp-hypers}
\end{table*}

\begin{table*}[h]
    \centering
    \begin{tabular}{|l|c|}
        \hline
        \multicolumn{2}{|c|}{\textbf{Computing Infrastructure}} \\ \hline
        Machine Type & AWS EC2 - p2.16xlarge\\
        GPU Family & Tesla K80 \\
        CPU Family & Intel Xeon 2.30GHz \\
        CUDA Version & $11.0$ \\
        NVIDIA-Driver & $450.80.02$ \\  \hline
       \multicolumn{2}{|c|}{\textbf{Library Version}} \\ \hline
        Python & $3.8.5$ \\
        Numpy &  $1.20.1$ \\
        Gym & $0.18.0$ \\
        Pytorch & $1.8.0$ \\
        \hline
   \end{tabular}
    \caption{\textbf{Computing infrastructure and software libraries used in all experiments in this paper.}}
    \label{tab:table-compute-hypers}
\end{table*}
\clearpage
\section{Additional Experiments}\label{sec:app:addational-expr}
\paragraph{Prioritized Experience Replay (PER).} In the standard DQN~\citepsi{mnih2015human}, data are uniformly sampled from the reply buffer regardless of their importance. To further improve the performance of DQN, \citesi{schaul2016prioritized} proposed an effective way, called prioritized experience replay, to prioritize samples that are more conducive to sample-efficient learning. To further evaluate and situate DQNPro, we compare \algname{} using standard replay buffer against DQN with prioritized experience replay (called PER) on 15 Atari games. As \Figref{fig:main-per} shows our method outperforms PER on the majority of these 15 games. These results provide another data point that our method is a more effective approach for improving the performance of DQN while adding negligible computation cost relative to PER.

\begin{figure}
\centering\captionsetup[subfigure]{justification=centering}
\begin{subfigure}[t]{ .18\textwidth} 
\centering 
\includegraphics[width=\textwidth]{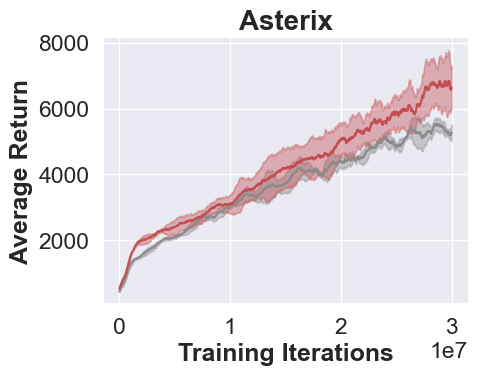} 
\label{fig:6_learning_curves_per_appendix/AsterixNoFrameskip-v0_5_learning_curves_appendix.png} 
\end{subfigure}% 
~ 
\begin{subfigure}[t]{ .18\textwidth} 
\centering 
\includegraphics[width=\textwidth]{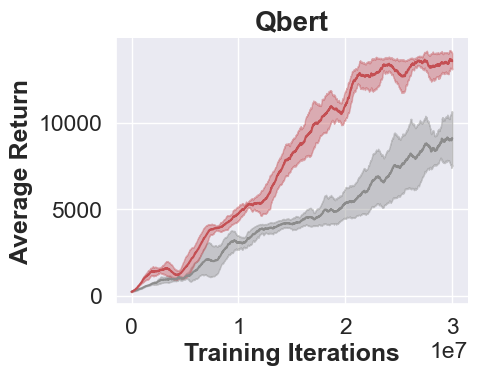} 
\label{fig:6_learning_curves_per_appendix/QbertNoFrameskip-v0_5_learning_curves_appendix.png} 
\end{subfigure}% 
~ 
\begin{subfigure}[t]{ .18\textwidth} 
\centering 
\includegraphics[width=\textwidth]{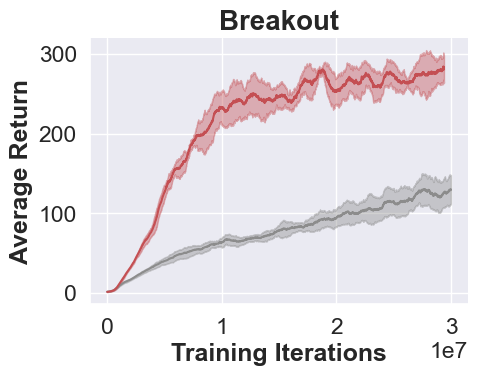} 
\label{fig:6_learning_curves_per_appendix/BreakoutNoFrameskip-v0_5_learning_curves_appendix.png} 
\end{subfigure}% 
~ 
\begin{subfigure}[t]{ .18\textwidth} 
\centering 
\includegraphics[width=\textwidth]{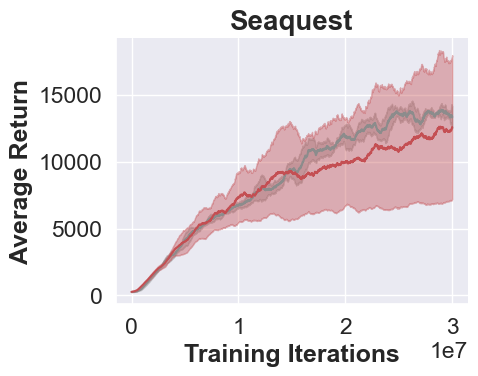} 
\label{fig:6_learning_curves_per_appendix/SeaquestNoFrameskip-v0_5_learning_curves_appendix.png} 
\end{subfigure}% 
~ 
\begin{subfigure}[t]{ .18\textwidth} 
\centering 
\includegraphics[width=\textwidth]{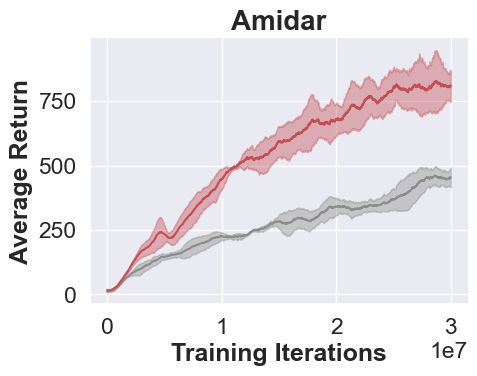} 
\label{fig:6_learning_curves_per_appendix/AmidarNoFrameskip-v0_5_learning_curves_appendix.png} 
\end{subfigure}% 

\begin{subfigure}[t]{ .18\textwidth} 
\centering 
\includegraphics[width=\textwidth]{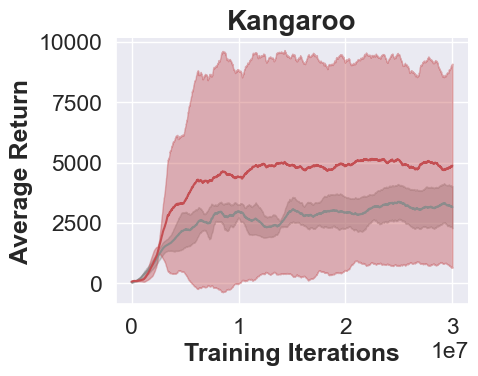} 
\label{fig:6_learning_curves_per_appendix/KangarooNoFrameskip-v0_5_learning_curves_appendix.png} 
\end{subfigure}% 
~ 
\begin{subfigure}[t]{ .18\textwidth} 
\centering 
\includegraphics[width=\textwidth]{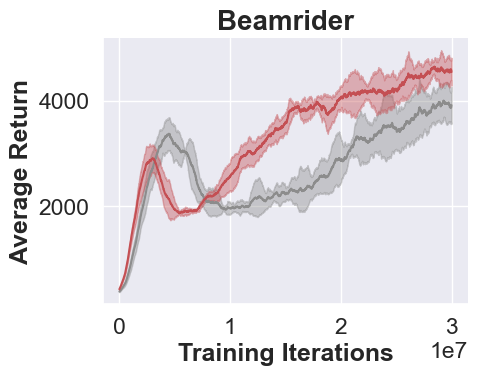} 
\label{fig:6_learning_curves_per_appendix/BeamRiderNoFrameskip-v0_5_learning_curves_appendix.png} 
\end{subfigure}% 
~ 
\begin{subfigure}[t]{ .18\textwidth} 
\centering 
\includegraphics[width=\textwidth]{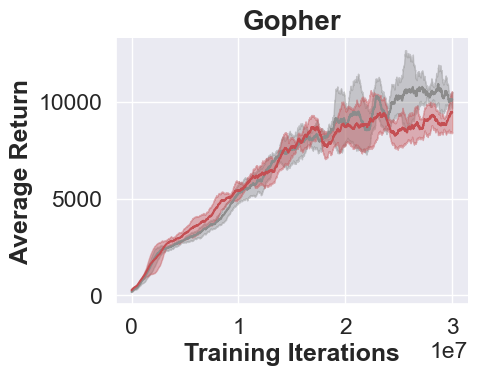} 
\label{fig:6_learning_curves_per_appendix/GopherNoFrameskip-v0_5_learning_curves_appendix.png} 
\end{subfigure}% 
~ 
\begin{subfigure}[t]{ .18\textwidth} 
\centering 
\includegraphics[width=\textwidth]{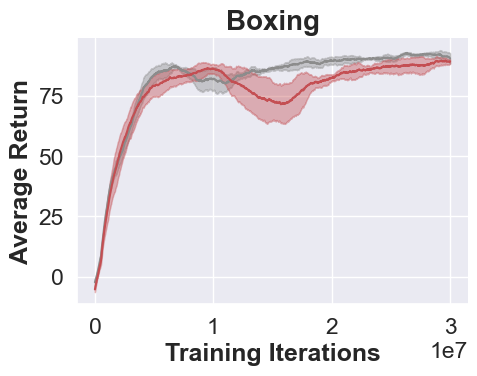} 
\label{fig:6_learning_curves_per_appendix/BoxingNoFrameskip-v0_5_learning_curves_appendix.png} 
\end{subfigure}% 
~ 
\begin{subfigure}[t]{ .18\textwidth} 
\centering 
\includegraphics[width=\textwidth]{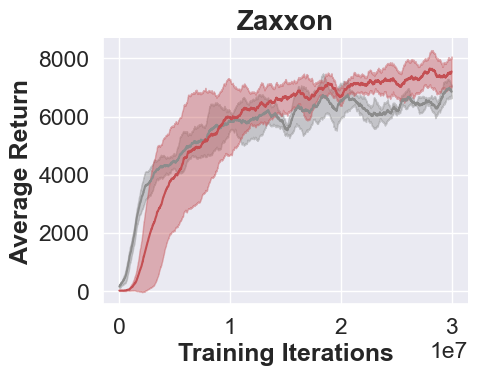} 
\label{fig:6_learning_curves_per_appendix/ZaxxonNoFrameskip-v0_5_learning_curves_appendix.png} 
\end{subfigure}% 

\begin{subfigure}[t]{ .18\textwidth} 
\centering 
\includegraphics[width=\textwidth]{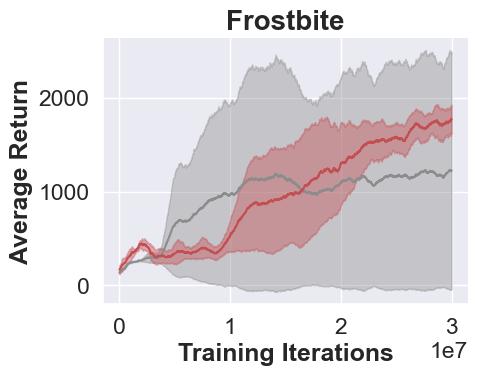} 
\label{fig:6_learning_curves_per_appendix/FrostbiteNoFrameskip-v0_5_learning_curves_appendix.png} 
\end{subfigure}% 
~ 
\begin{subfigure}[t]{ .18\textwidth} 
\centering 
\includegraphics[width=\textwidth]{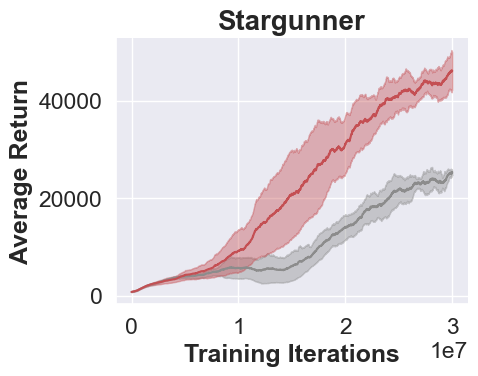} 
\label{fig:6_learning_curves_per_appendix/StarGunnerNoFrameskip-v0_5_learning_curves_appendix.png} 
\end{subfigure}% 
~ 
\begin{subfigure}[t]{ .18\textwidth} 
\centering 
\includegraphics[width=\textwidth]{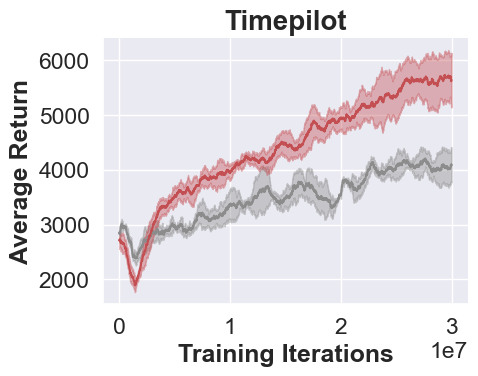} 
\label{fig:6_learning_curves_per_appendix/TimePilotNoFrameskip-v0_5_learning_curves_appendix.png} 
\end{subfigure}% 
~ 
\begin{subfigure}[t]{ .18\textwidth} 
\centering 
\includegraphics[width=\textwidth]{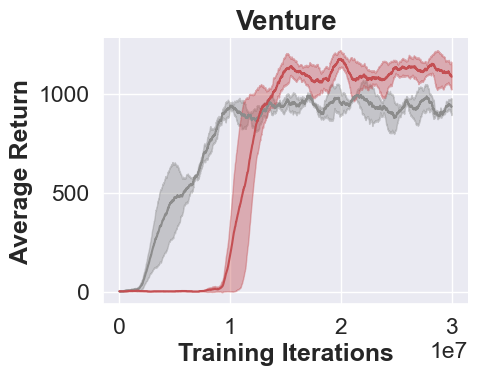} 
\label{fig:6_learning_curves_per_appendix/VentureNoFrameskip-v0_5_learning_curves_appendix.png} 
\end{subfigure}% 
~ 
\begin{subfigure}[t]{ .18\textwidth} 
\centering 
\includegraphics[width=\textwidth]{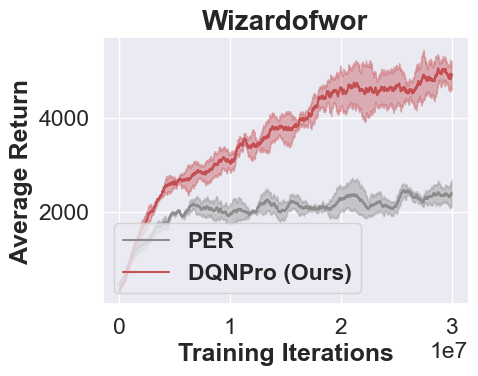} 
\label{fig:6_learning_curves_per_appendix/WizardOfWorNoFrameskip-v0_5_learning_curves_appendix.png} 
\end{subfigure}% 

\caption{
\textbf{Learning curves for DQN with prioritized experience replay (PER) (gary) and \algname{} (red)} on 15 Atari games. X-axis indicates the number of steps from the environment used in training and Y-axis shows average undiscounted return.
%A comparison between DQNPro and Prioritized Experience Replay (PER) citation zzz.
} 
\label{fig:main-per} 
\end{figure} 

\begin{figure}[t]
\centering
\begin{subfigure}[b]{.9\textwidth}
   \includegraphics[width=1\linewidth]{1_main_comparison/pddqn_ddqn.pdf}
\end{subfigure}
\caption{\textbf{Performance gain for D\algname{} over the original DDQN in term of the final performance.} Results are averaged over four random seeds.The y-axis is scaled logarithmically.}
\label{fig:ddqn}
\end{figure}
\section{Learning curves}\label{sec:app:learning-curves}
In this section, we provide all learning curves for the experiments described in \Secref{sec:results} of the main text. Specifically, \Figref{fig:main} shows learning curves for DQN and \algname{} and \Figref{fig:ddqn} and \Figref{fig:main_ddqn} show results comparing D\algname{} against DDQN for 40 Atari-2600 games.

\begin{figure}
\centering\captionsetup[subfigure]{justification=centering}
\begin{subfigure}[t]{ .18\textwidth} 
\centering 
\includegraphics[width=\textwidth]{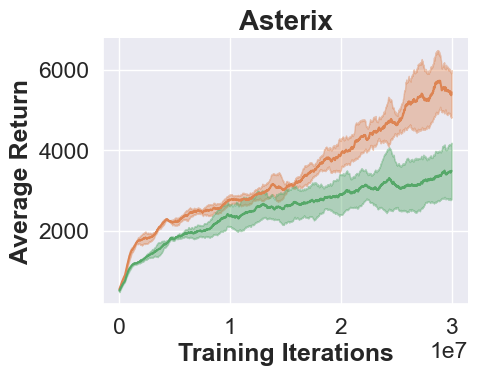} 
\label{fig:5_learning_curves_appendix/AsterixNoFrameskip-v0_5_learning_curves_appendix.png} 
\end{subfigure}% 
~ 
\begin{subfigure}[t]{ .18\textwidth} 
\centering 
\includegraphics[width=\textwidth]{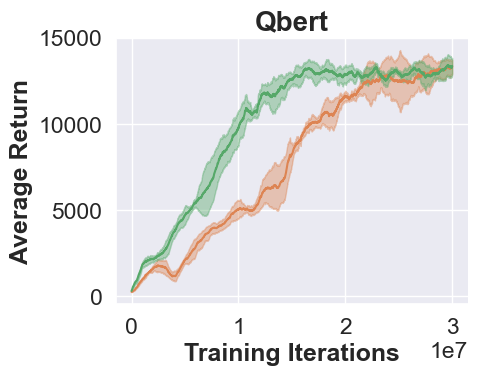} 
\label{fig:5_learning_curves_appendix/QbertNoFrameskip-v0_5_learning_curves_appendix.png} 
\end{subfigure}% 
~ 
\begin{subfigure}[t]{ .18\textwidth} 
\centering 
\includegraphics[width=\textwidth]{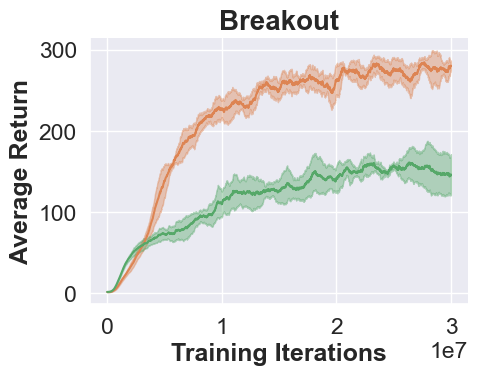} 
\label{fig:5_learning_curves_appendix/BreakoutNoFrameskip-v0_5_learning_curves_appendix.png} 
\end{subfigure}% 
~ 
\begin{subfigure}[t]{ .18\textwidth} 
\centering 
\includegraphics[width=\textwidth]{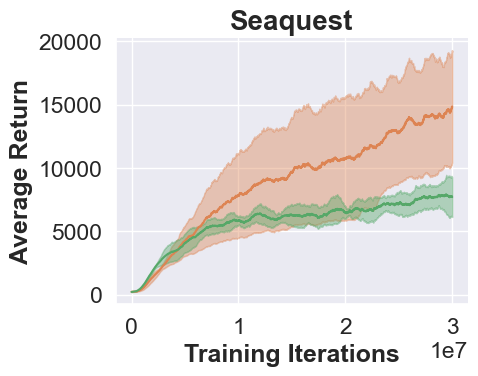} 
\label{fig:5_learning_curves_appendix/SeaquestNoFrameskip-v0_5_learning_curves_appendix.png} 
\end{subfigure}% 
~ 
\begin{subfigure}[t]{ .18\textwidth} 
\centering 
\includegraphics[width=\textwidth]{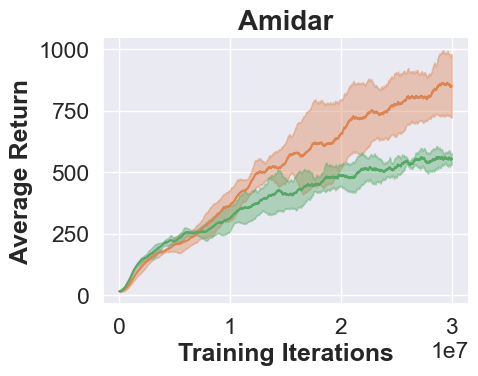} 
\label{fig:5_learning_curves_appendix/AmidarNoFrameskip-v0_5_learning_curves_appendix.png} 
\end{subfigure}% 

\begin{subfigure}[t]{ .18\textwidth} 
\centering 
\includegraphics[width=\textwidth]{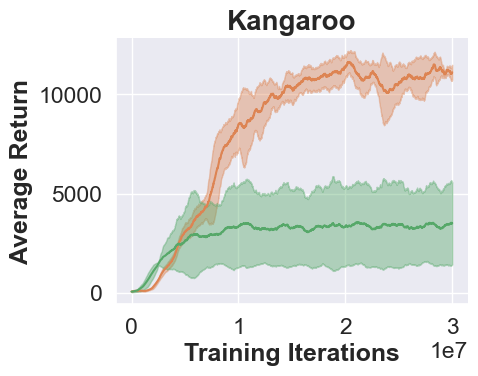} 
\label{fig:5_learning_curves_appendix/KangarooNoFrameskip-v0_5_learning_curves_appendix.png} 
\end{subfigure}% 
~ 
\begin{subfigure}[t]{ .18\textwidth} 
\centering 
\includegraphics[width=\textwidth]{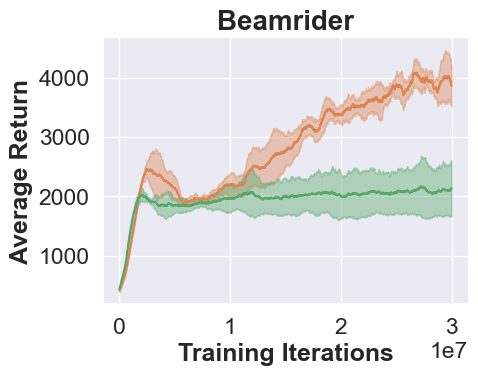} 
\label{fig:5_learning_curves_appendix/BeamRiderNoFrameskip-v0_5_learning_curves_appendix.png} 
\end{subfigure}% 
~ 
\begin{subfigure}[t]{ .18\textwidth} 
\centering 
\includegraphics[width=\textwidth]{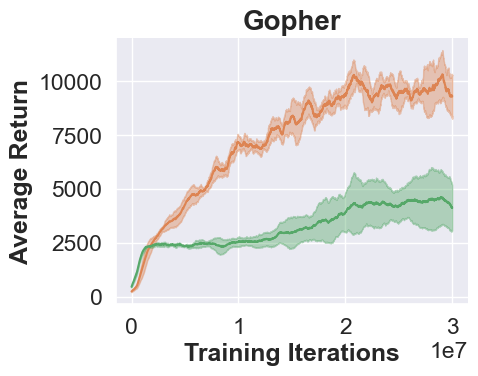} 
\label{fig:5_learning_curves_appendix/GopherNoFrameskip-v0_5_learning_curves_appendix.png} 
\end{subfigure}% 
~ 
\begin{subfigure}[t]{ .18\textwidth} 
\centering 
\includegraphics[width=\textwidth]{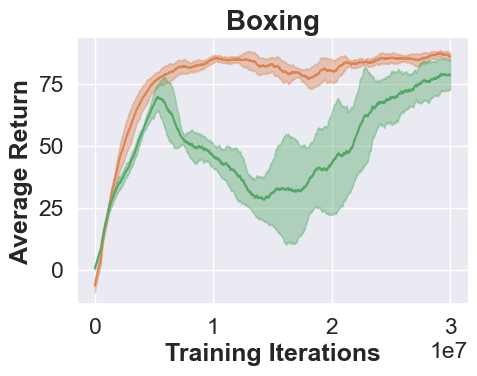} 
\label{fig:5_learning_curves_appendix/BoxingNoFrameskip-v0_5_learning_curves_appendix.png} 
\end{subfigure}% 
~ 
\begin{subfigure}[t]{ .18\textwidth} 
\centering 
\includegraphics[width=\textwidth]{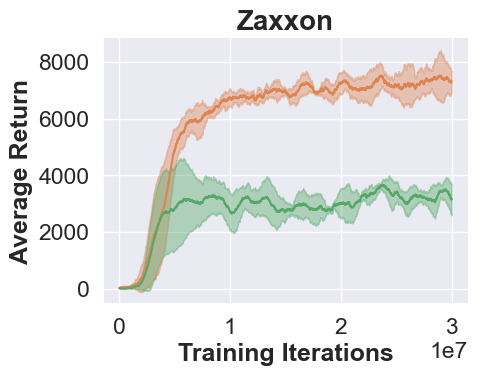} 
\label{fig:5_learning_curves_appendix/ZaxxonNoFrameskip-v0_5_learning_curves_appendix.png} 
\end{subfigure}% 

\begin{subfigure}[t]{ .18\textwidth} 
\centering 
\includegraphics[width=\textwidth]{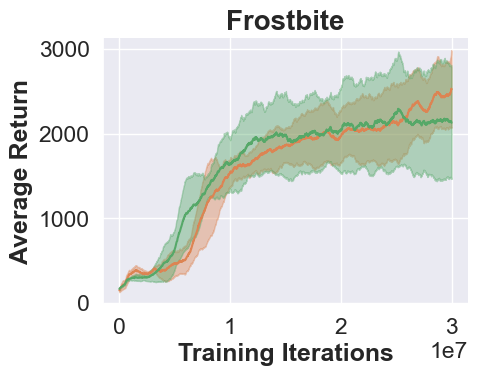} 
\label{fig:5_learning_curves_appendix/FrostbiteNoFrameskip-v0_5_learning_curves_appendix.png} 
\end{subfigure}% 
~ 
\begin{subfigure}[t]{ .18\textwidth} 
\centering 
\includegraphics[width=\textwidth]{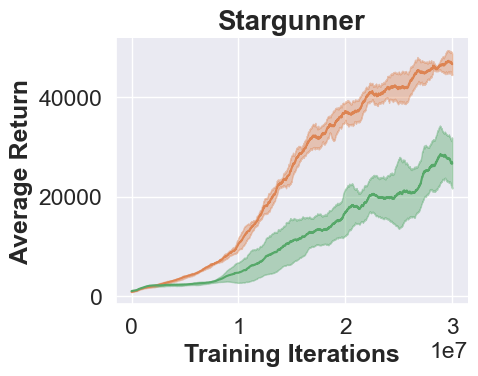} 
\label{fig:5_learning_curves_appendix/StarGunnerNoFrameskip-v0_5_learning_curves_appendix.png} 
\end{subfigure}% 
~ 
\begin{subfigure}[t]{ .18\textwidth} 
\centering 
\includegraphics[width=\textwidth]{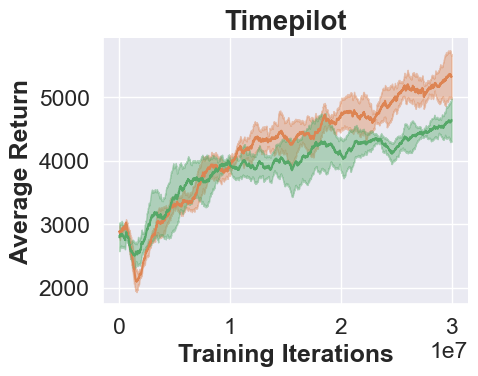} 
\label{fig:5_learning_curves_appendix/TimePilotNoFrameskip-v0_5_learning_curves_appendix.png} 
\end{subfigure}% 
~ 
\begin{subfigure}[t]{ .18\textwidth} 
\centering 
\includegraphics[width=\textwidth]{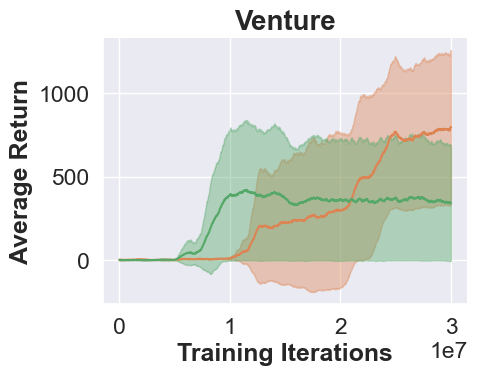} 
\label{fig:5_learning_curves_appendix/VentureNoFrameskip-v0_5_learning_curves_appendix.png} 
\end{subfigure}% 
~ 
\begin{subfigure}[t]{ .18\textwidth} 
\centering 
\includegraphics[width=\textwidth]{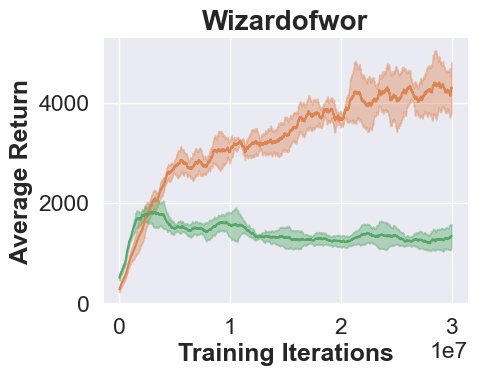} 
\label{fig:5_learning_curves_appendix/WizardOfWorNoFrameskip-v0_5_learning_curves_appendix.png} 
\end{subfigure}% 

\begin{subfigure}[t]{ .18\textwidth} 
\centering 
\includegraphics[width=\textwidth]{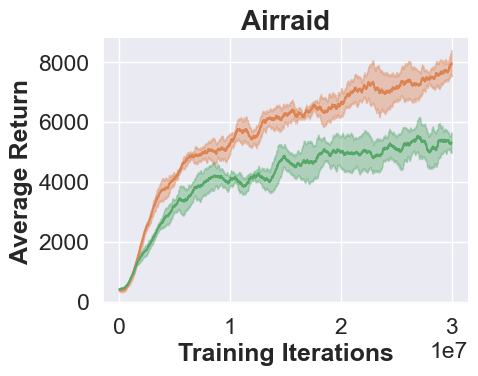} 
\label{fig:5_learning_curves_appendix/AirRaidNoFrameskip-v0_5_learning_curves_appendix.png} 
\end{subfigure}% 
~ 
\begin{subfigure}[t]{ .18\textwidth} 
\centering 
\includegraphics[width=\textwidth]{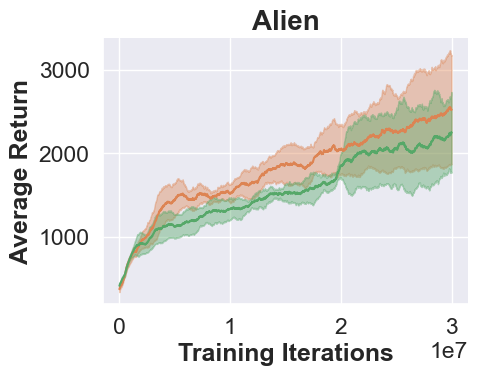} 
\label{fig:5_learning_curves_appendix/AlienNoFrameskip-v0_5_learning_curves_appendix.png} 
\end{subfigure}% 
~ 
\begin{subfigure}[t]{ .18\textwidth} 
\centering 
\includegraphics[width=\textwidth]{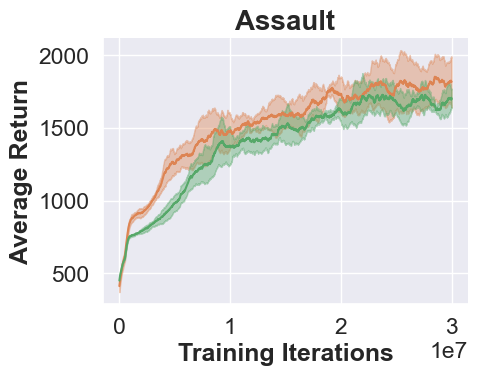} 
\label{fig:5_learning_curves_appendix/AssaultNoFrameskip-v0_5_learning_curves_appendix.png} 
\end{subfigure}% 
~ 
\begin{subfigure}[t]{ .18\textwidth} 
\centering 
\includegraphics[width=\textwidth]{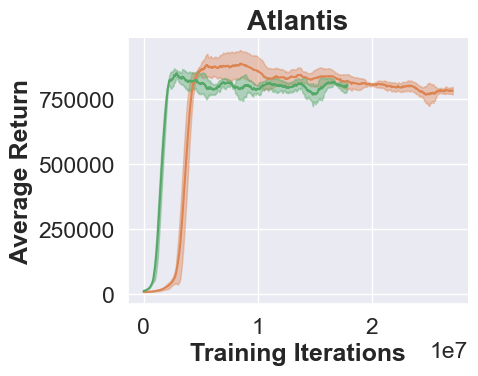} 
\label{fig:5_learning_curves_appendix/AtlantisNoFrameskip-v0_5_learning_curves_appendix.png} 
\end{subfigure}% 
~ 
\begin{subfigure}[t]{ .18\textwidth} 
\centering 
\includegraphics[width=\textwidth]{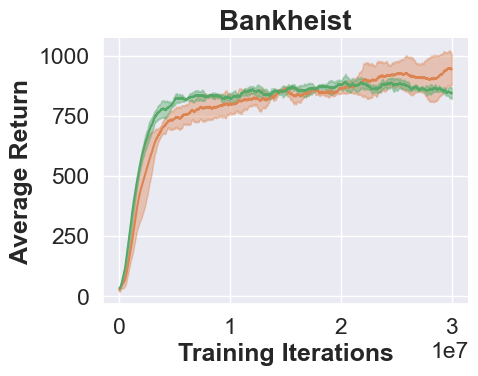} 
\label{fig:5_learning_curves_appendix/BankHeistNoFrameskip-v0_5_learning_curves_appendix.png} 
\end{subfigure}% 

\begin{subfigure}[t]{ .18\textwidth} 
\centering 
\includegraphics[width=\textwidth]{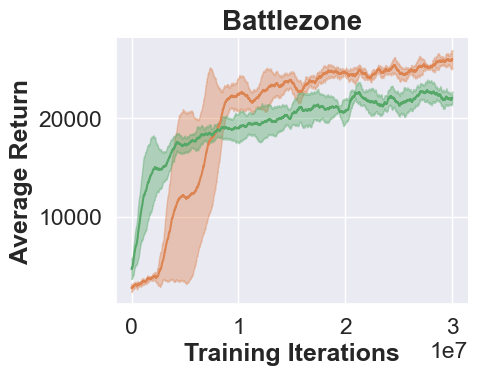} 
\label{fig:5_learning_curves_appendix/BattleZoneNoFrameskip-v0_5_learning_curves_appendix.png} 
\end{subfigure}% 
~ 
\begin{subfigure}[t]{ .18\textwidth} 
\centering 
\includegraphics[width=\textwidth]{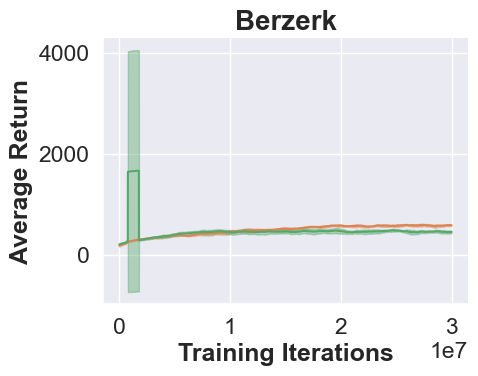} 
\label{fig:5_learning_curves_appendix/BerzerkNoFrameskip-v0_5_learning_curves_appendix.png} 
\end{subfigure}% 
~ 
\begin{subfigure}[t]{ .18\textwidth} 
\centering 
\includegraphics[width=\textwidth]{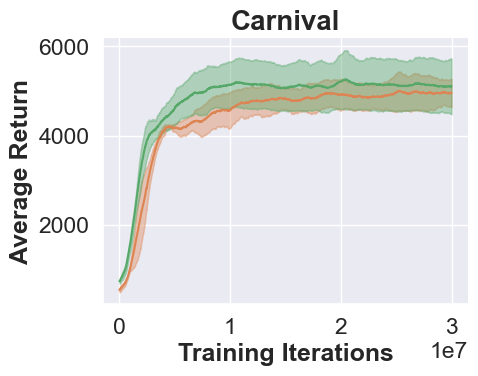} 
\label{fig:5_learning_curves_appendix/CarnivalNoFrameskip-v0_5_learning_curves_appendix.png} 
\end{subfigure}% 
~ 
\begin{subfigure}[t]{ .18\textwidth} 
\centering 
\includegraphics[width=\textwidth]{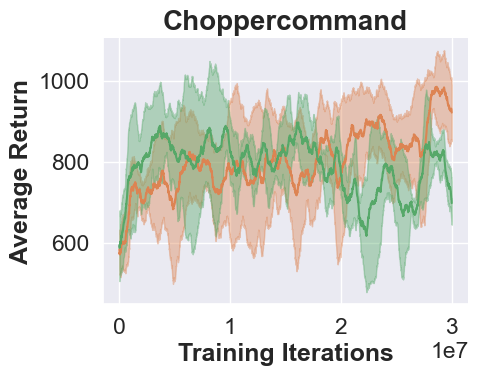} 
\label{fig:5_learning_curves_appendix/ChopperCommandNoFrameskip-v0_5_learning_curves_appendix.png} 
\end{subfigure}% 
~ 
\begin{subfigure}[t]{ .18\textwidth} 
\centering 
\includegraphics[width=\textwidth]{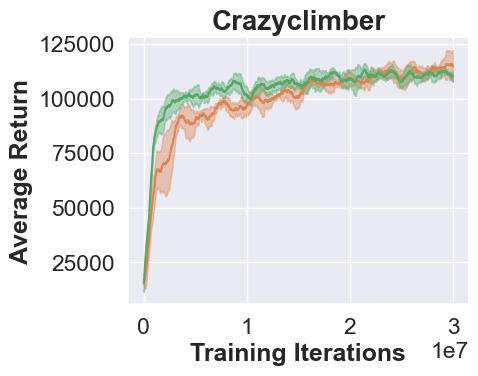} 
\label{fig:5_learning_curves_appendix/CrazyClimberNoFrameskip-v0_5_learning_curves_appendix.png} 
\end{subfigure}% 

\begin{subfigure}[t]{ .18\textwidth} 
\centering 
\includegraphics[width=\textwidth]{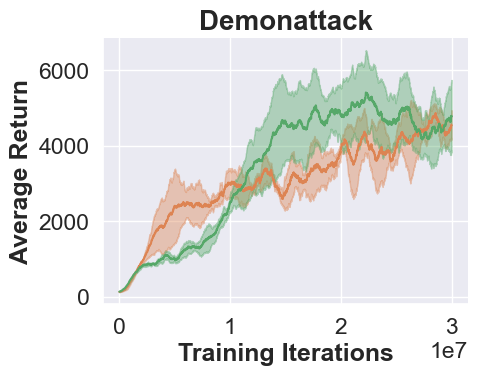} 
\label{fig:5_learning_curves_appendix/DemonAttackNoFrameskip-v0_5_learning_curves_appendix.png} 
\end{subfigure}% 
~ 
\begin{subfigure}[t]{ .18\textwidth} 
\centering 
\includegraphics[width=\textwidth]{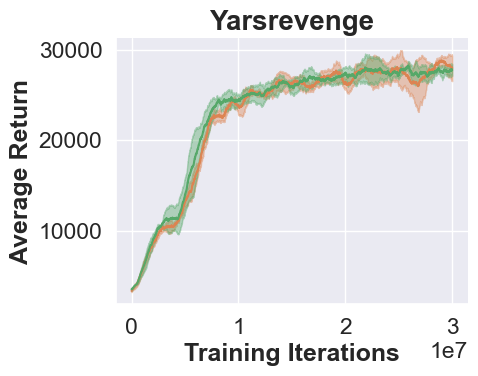} 
\label{fig:5_learning_curves_appendix/YarsRevengeNoFrameskip-v0_5_learning_curves_appendix.png} 
\end{subfigure}% 
~ 
\begin{subfigure}[t]{ .18\textwidth} 
\centering 
\includegraphics[width=\textwidth]{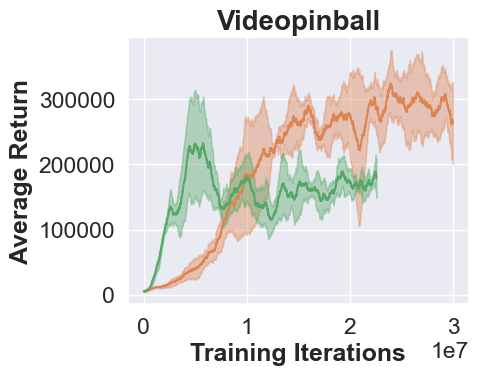} 
\label{fig:5_learning_curves_appendix/VideoPinballNoFrameskip-v0_5_learning_curves_appendix.png} 
\end{subfigure}% 
~ 
\begin{subfigure}[t]{ .18\textwidth} 
\centering 
\includegraphics[width=\textwidth]{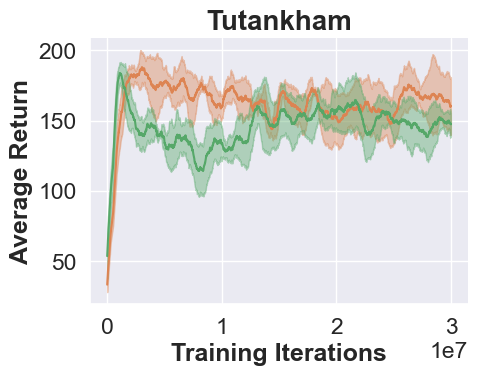} 
\label{fig:5_learning_curves_appendix/TutankhamNoFrameskip-v0_5_learning_curves_appendix.png} 
\end{subfigure}% 
~ 
\begin{subfigure}[t]{ .18\textwidth} 
\centering 
\includegraphics[width=\textwidth]{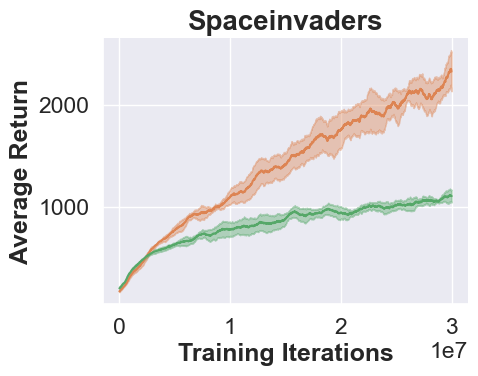} 
\label{fig:5_learning_curves_appendix/SpaceInvadersNoFrameskip-v0_5_learning_curves_appendix.png} 
\end{subfigure}% 

\begin{subfigure}[t]{ .18\textwidth} 
\centering 
\includegraphics[width=\textwidth]{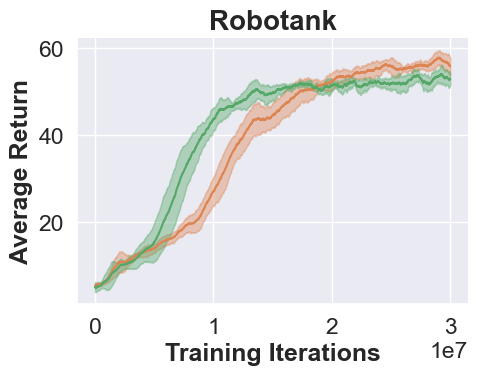} 
\label{fig:5_learning_curves_appendix/RobotankNoFrameskip-v0_5_learning_curves_appendix.png} 
\end{subfigure}% 
~ 
\begin{subfigure}[t]{ .18\textwidth} 
\centering 
\includegraphics[width=\textwidth]{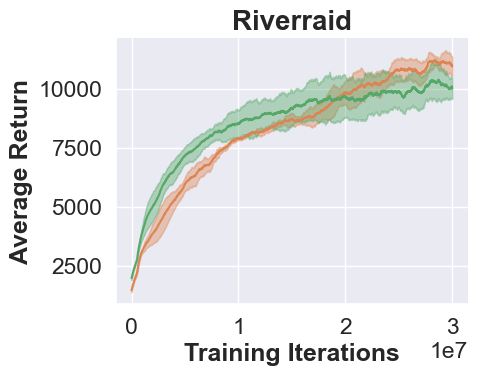} 
\label{fig:5_learning_curves_appendix/RiverraidNoFrameskip-v0_5_learning_curves_appendix.png} 
\end{subfigure}% 
~ 
\begin{subfigure}[t]{ .18\textwidth} 
\centering 
\includegraphics[width=\textwidth]{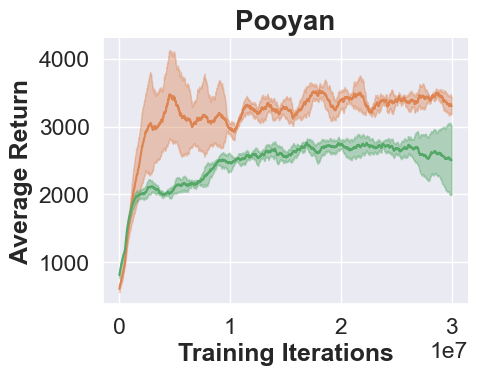} 
\label{fig:5_learning_curves_appendix/PooyanNoFrameskip-v0_5_learning_curves_appendix.png} 
\end{subfigure}% 
~ 
\begin{subfigure}[t]{ .18\textwidth} 
\centering 
\includegraphics[width=\textwidth]{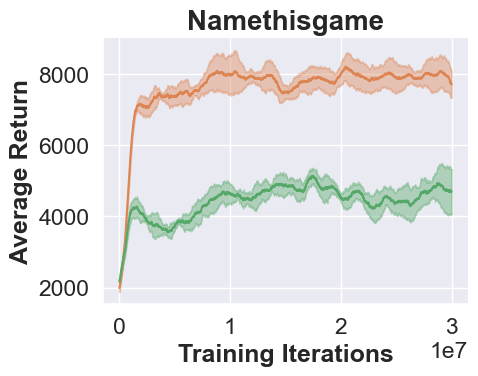} 
\label{fig:5_learning_curves_appendix/NameThisGameNoFrameskip-v0_5_learning_curves_appendix.png} 
\end{subfigure}% 
~ 
\begin{subfigure}[t]{ .18\textwidth} 
\centering 
\includegraphics[width=\textwidth]{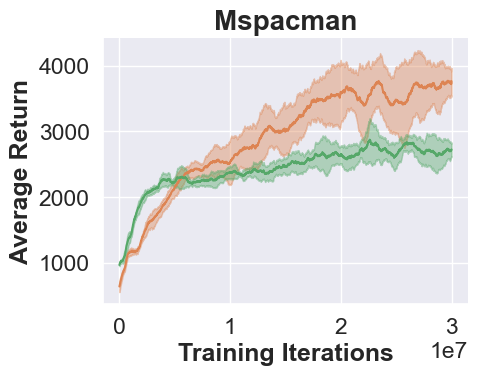} 
\label{fig:5_learning_curves_appendix/MsPacmanNoFrameskip-v0_5_learning_curves_appendix.png} 
\end{subfigure}% 

\begin{subfigure}[t]{ .18\textwidth} 
\centering 
\includegraphics[width=\textwidth]{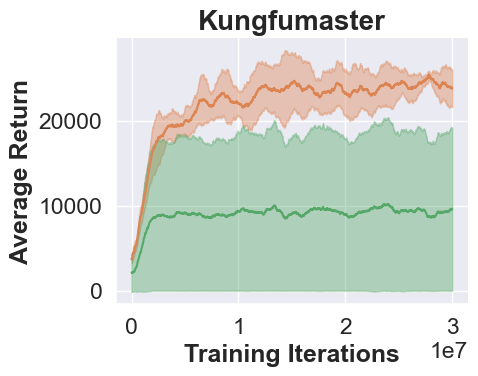} 
\label{fig:5_learning_curves_appendix/KungFuMasterNoFrameskip-v0_5_learning_curves_appendix.png} 
\end{subfigure}% 
~ 
\begin{subfigure}[t]{ .18\textwidth} 
\centering 
\includegraphics[width=\textwidth]{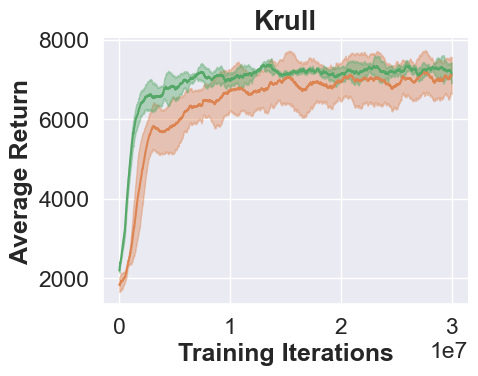} 
\label{fig:5_learning_curves_appendix/KrullNoFrameskip-v0_5_learning_curves_appendix.png} 
\end{subfigure}% 
~ 
\begin{subfigure}[t]{ .18\textwidth} 
\centering 
\includegraphics[width=\textwidth]{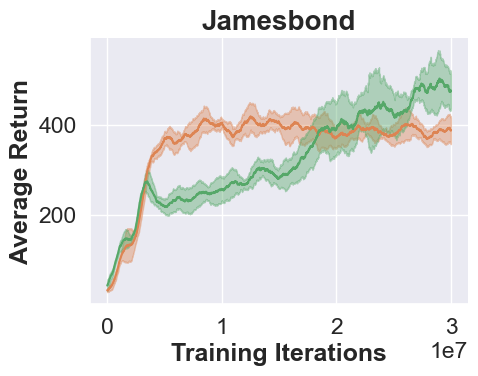} 
\label{fig:5_learning_curves_appendix/JamesbondNoFrameskip-v0_5_learning_curves_appendix.png} 
\end{subfigure}% 
~ 
\begin{subfigure}[t]{ .18\textwidth} 
\centering 
\includegraphics[width=\textwidth]{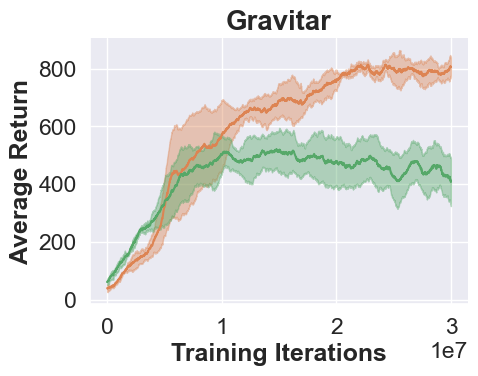} 
\label{fig:5_learning_curves_appendix/GravitarNoFrameskip-v0_5_learning_curves_appendix.png} 
\end{subfigure}% 
~ 
\begin{subfigure}[t]{ .18\textwidth} 
\centering 
\includegraphics[width=\textwidth]{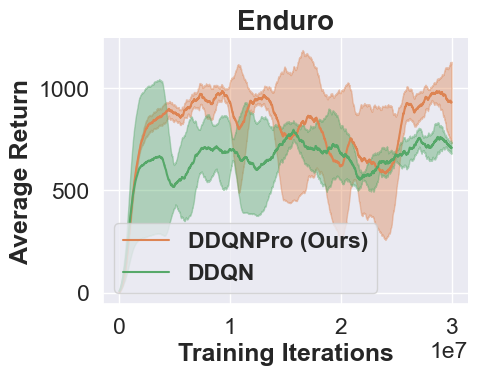} 
\label{fig:5_learning_curves_appendix/EnduroNoFrameskip-v0_5_learning_curves_appendix.png} 
\end{subfigure}% 

\caption{\textbf{Learning curves for DDQN (green) and D\algname{} (orange)} on 40 Atari games. X-axis indicates the number of steps from the environment used in training and Y-axis shows average undiscounted return.}
%A comparison between DDQNPro and DDQN in terms of asymptotic performance.
 
\label{fig:main_ddqn} 
\end{figure}

\begin{figure}
\centering\captionsetup[subfigure]{justification=centering}
\begin{subfigure}[t]{ .18\textwidth} 
\centering 
\includegraphics[width=\textwidth]{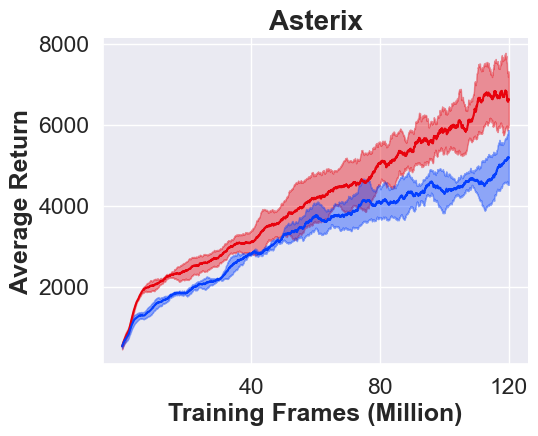} 
\label{fig:4_learning_curves_appendix/AsterixNoFrameskip-v0_4_learning_curves_appendix.png} 
\end{subfigure}% 
~ 
\begin{subfigure}[t]{ .18\textwidth} 
\centering 
\includegraphics[width=\textwidth]{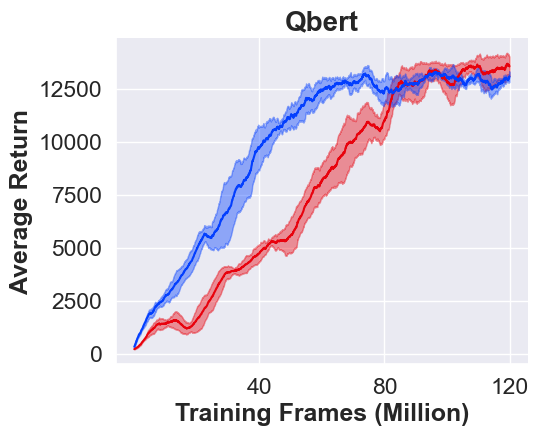} 
\label{fig:4_learning_curves_appendix/QbertNoFrameskip-v0_4_learning_curves_appendix.png} 
\end{subfigure}% 
~ 
\begin{subfigure}[t]{ .18\textwidth} 
\centering 
\includegraphics[width=\textwidth]{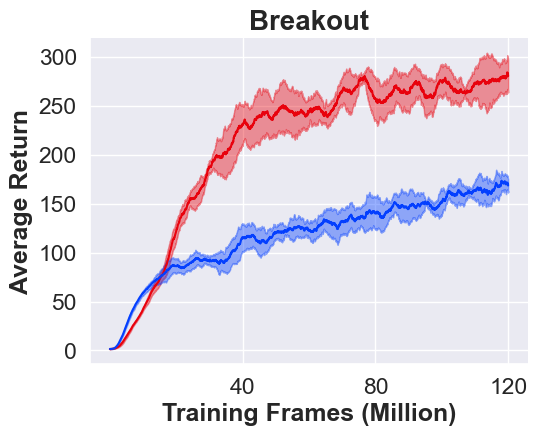} 
\label{fig:4_learning_curves_appendix/BreakoutNoFrameskip-v0_4_learning_curves_appendix.png} 
\end{subfigure}% 
~ 
\begin{subfigure}[t]{ .18\textwidth} 
\centering 
\includegraphics[width=\textwidth]{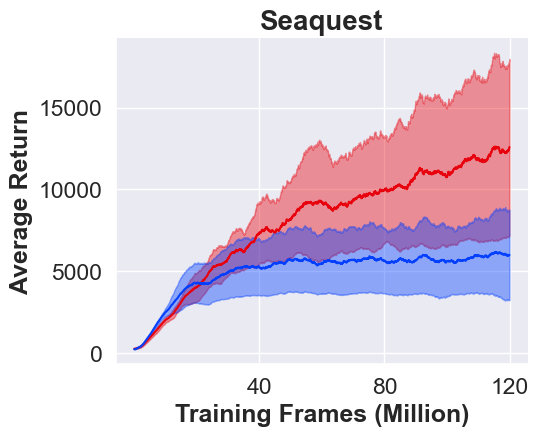} 
\label{fig:4_learning_curves_appendix/SeaquestNoFrameskip-v0_4_learning_curves_appendix.png} 
\end{subfigure}% 
~ 
\begin{subfigure}[t]{ .18\textwidth} 
\centering 
\includegraphics[width=\textwidth]{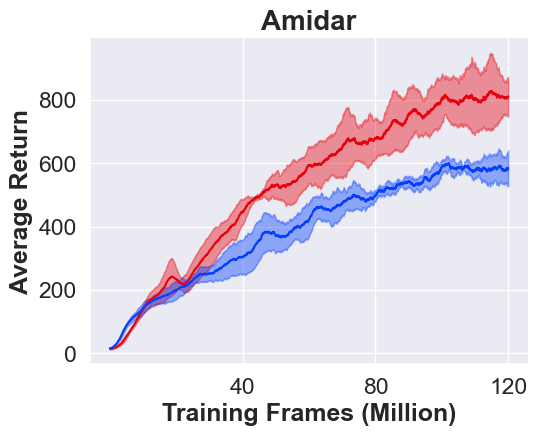} 
\label{fig:4_learning_curves_appendix/AmidarNoFrameskip-v0_4_learning_curves_appendix.png} 
\end{subfigure}% 

\begin{subfigure}[t]{ .18\textwidth} 
\centering 
\includegraphics[width=\textwidth]{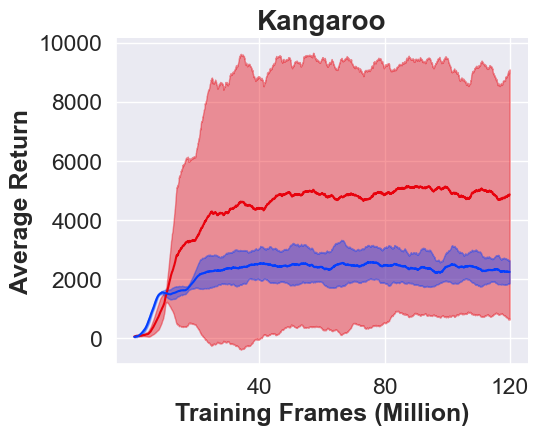} 
\label{fig:4_learning_curves_appendix/KangarooNoFrameskip-v0_4_learning_curves_appendix.png} 
\end{subfigure}% 
~ 
\begin{subfigure}[t]{ .18\textwidth} 
\centering 
\includegraphics[width=\textwidth]{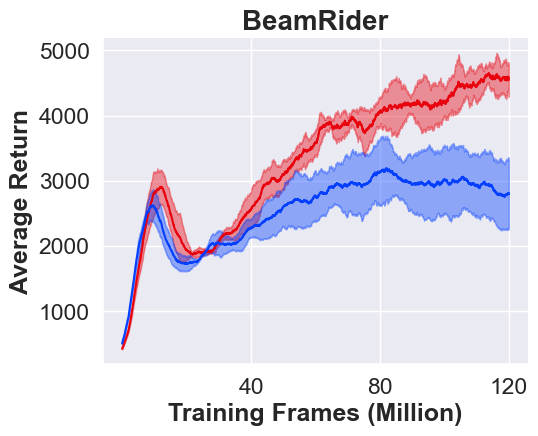} 
\label{fig:4_learning_curves_appendix/BeamRiderNoFrameskip-v0_4_learning_curves_appendix.png} 
\end{subfigure}% 
~ 
\begin{subfigure}[t]{ .18\textwidth} 
\centering 
\includegraphics[width=\textwidth]{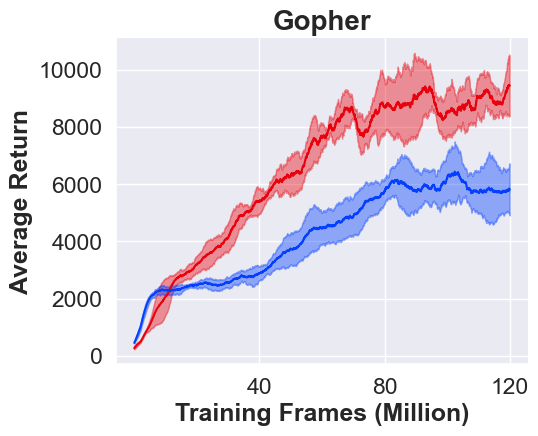} 
\label{fig:4_learning_curves_appendix/GopherNoFrameskip-v0_4_learning_curves_appendix.png} 
\end{subfigure}% 
~ 
\begin{subfigure}[t]{ .18\textwidth} 
\centering 
\includegraphics[width=\textwidth]{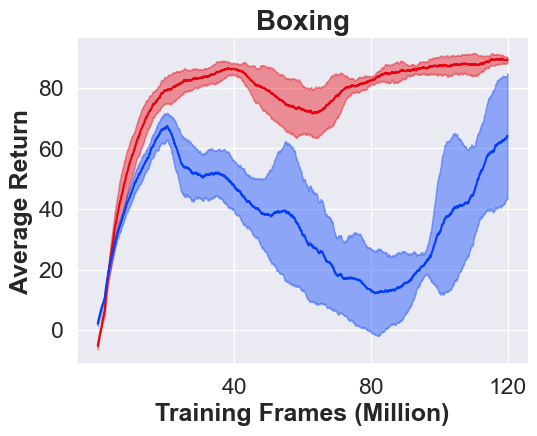} 
\label{fig:4_learning_curves_appendix/BoxingNoFrameskip-v0_4_learning_curves_appendix.png} 
\end{subfigure}% 
~ 
\begin{subfigure}[t]{ .18\textwidth} 
\centering 
\includegraphics[width=\textwidth]{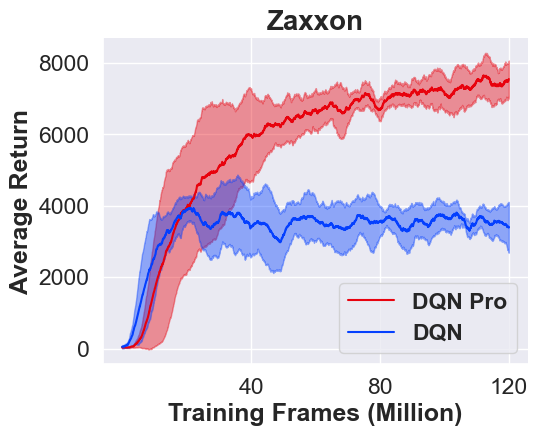} 
\label{fig:4_learning_curves_appendix/ZaxxonNoFrameskip-v0_4_learning_curves_appendix.png} 
\end{subfigure}% 

\begin{subfigure}[t]{ .18\textwidth} 
\centering 
\includegraphics[width=\textwidth]{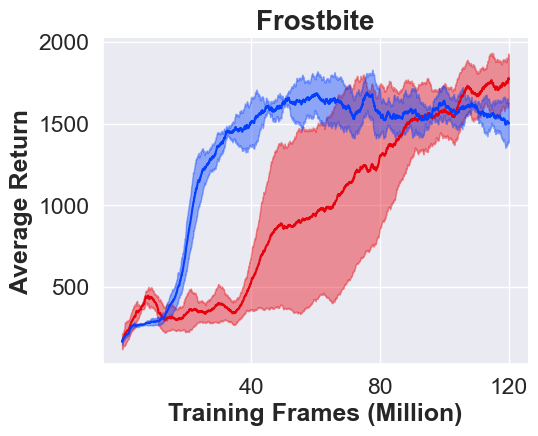} 
\label{fig:4_learning_curves_appendix/FrostbiteNoFrameskip-v0_4_learning_curves_appendix.png} 
\end{subfigure}% 
~ 
\begin{subfigure}[t]{ .18\textwidth} 
\centering 
\includegraphics[width=\textwidth]{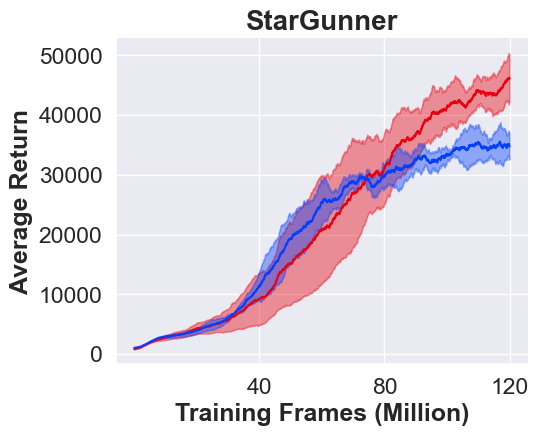} 
\label{fig:4_learning_curves_appendix/StarGunnerNoFrameskip-v0_4_learning_curves_appendix.png} 
\end{subfigure}% 
~ 
\begin{subfigure}[t]{ .18\textwidth} 
\centering 
\includegraphics[width=\textwidth]{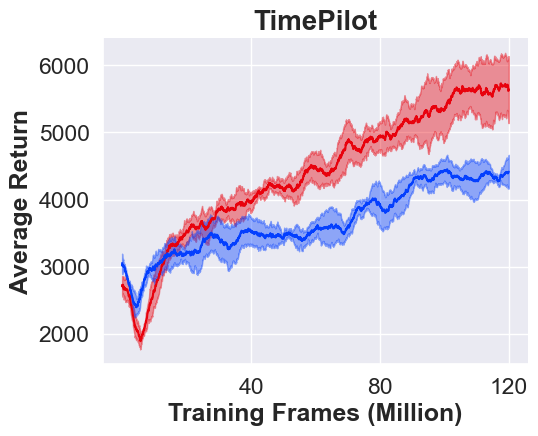} 
\label{fig:4_learning_curves_appendix/TimePilotNoFrameskip-v0_4_learning_curves_appendix.png} 
\end{subfigure}% 
~ 
\begin{subfigure}[t]{ .18\textwidth} 
\centering 
\includegraphics[width=\textwidth]{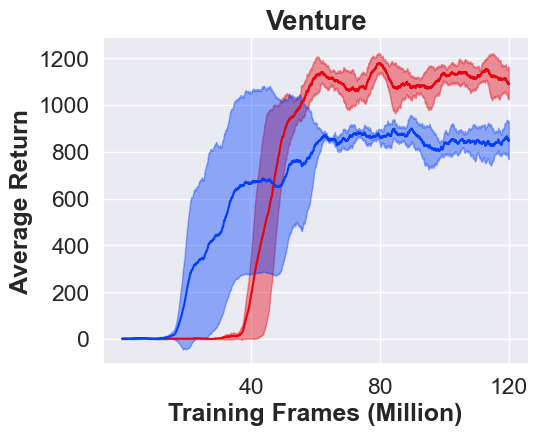} 
\label{fig:4_learning_curves_appendix/VentureNoFrameskip-v0_4_learning_curves_appendix.png} 
\end{subfigure}% 
~ 
\begin{subfigure}[t]{ .18\textwidth} 
\centering 
\includegraphics[width=\textwidth]{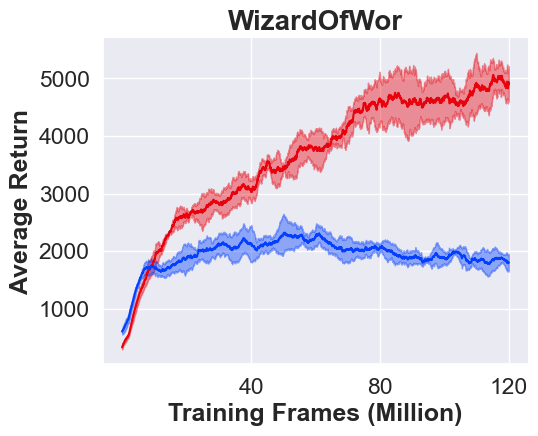} 
\label{fig:4_learning_curves_appendix/WizardOfWorNoFrameskip-v0_4_learning_curves_appendix.png} 
\end{subfigure}% 

\begin{subfigure}[t]{ .18\textwidth} 
\centering 
\includegraphics[width=\textwidth]{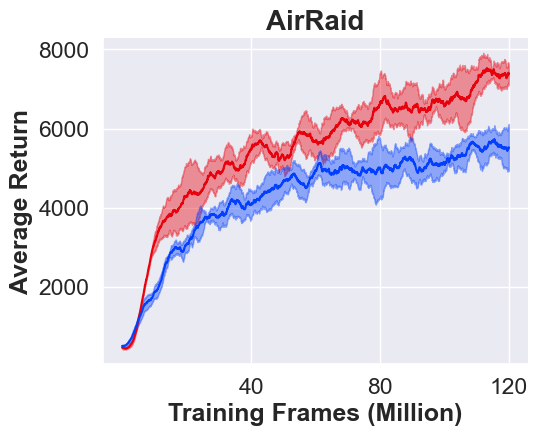} 
\label{fig:4_learning_curves_appendix/AirRaidNoFrameskip-v0_4_learning_curves_appendix.png} 
\end{subfigure}% 
~ 
\begin{subfigure}[t]{ .18\textwidth} 
\centering 
\includegraphics[width=\textwidth]{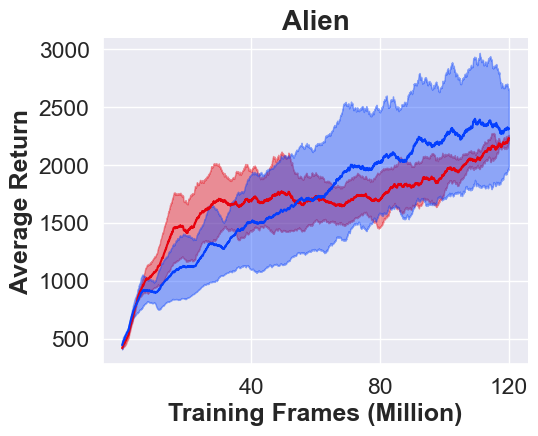} 
\label{fig:4_learning_curves_appendix/AlienNoFrameskip-v0_4_learning_curves_appendix.png} 
\end{subfigure}% 
~ 
\begin{subfigure}[t]{ .18\textwidth} 
\centering 
\includegraphics[width=\textwidth]{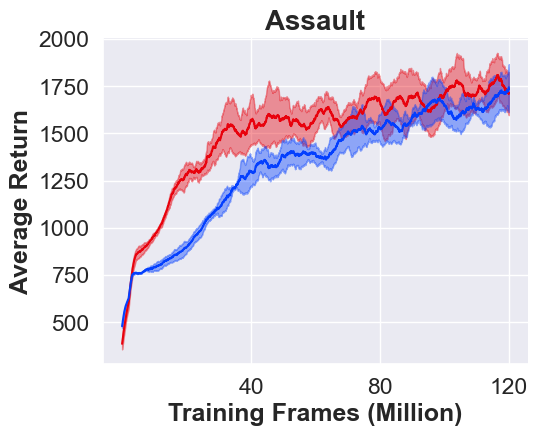} 
\label{fig:4_learning_curves_appendix/AssaultNoFrameskip-v0_4_learning_curves_appendix.png} 
\end{subfigure}% 
~ 
\begin{subfigure}[t]{ .18\textwidth} 
\centering 
\includegraphics[width=\textwidth]{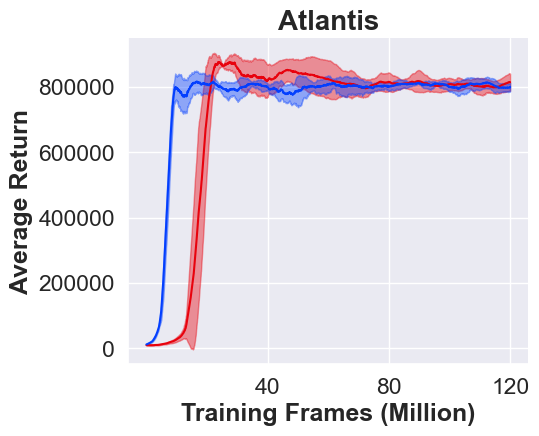} 
\label{fig:4_learning_curves_appendix/AtlantisNoFrameskip-v0_4_learning_curves_appendix.png} 
\end{subfigure}% 
~ 
\begin{subfigure}[t]{ .18\textwidth} 
\centering 
\includegraphics[width=\textwidth]{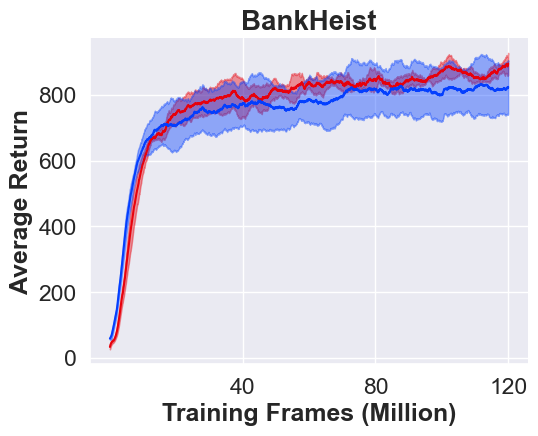} 
\label{fig:4_learning_curves_appendix/BankHeistNoFrameskip-v0_4_learning_curves_appendix.png} 
\end{subfigure}% 

\begin{subfigure}[t]{ .18\textwidth} 
\centering 
\includegraphics[width=\textwidth]{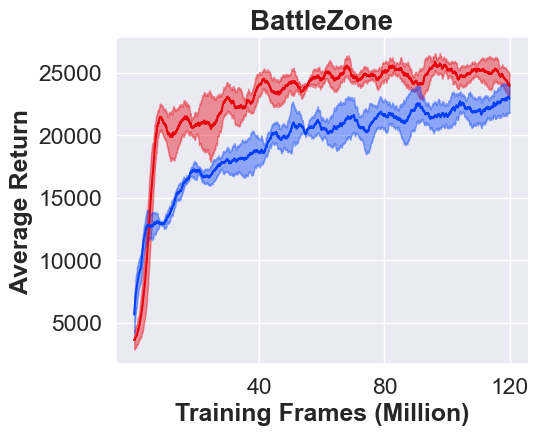} 
\label{fig:4_learning_curves_appendix/BattleZoneNoFrameskip-v0_4_learning_curves_appendix.png} 
\end{subfigure}% 
~ 
\begin{subfigure}[t]{ .18\textwidth} 
\centering 
\includegraphics[width=\textwidth]{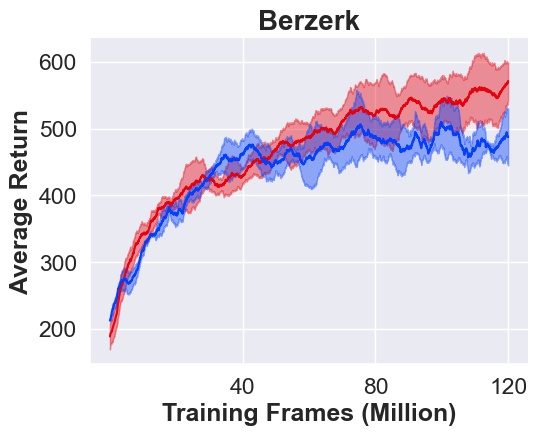} 
\label{fig:4_learning_curves_appendix/BerzerkNoFrameskip-v0_4_learning_curves_appendix.png} 
\end{subfigure}% 
~ 
\begin{subfigure}[t]{ .18\textwidth} 
\centering 
\includegraphics[width=\textwidth]{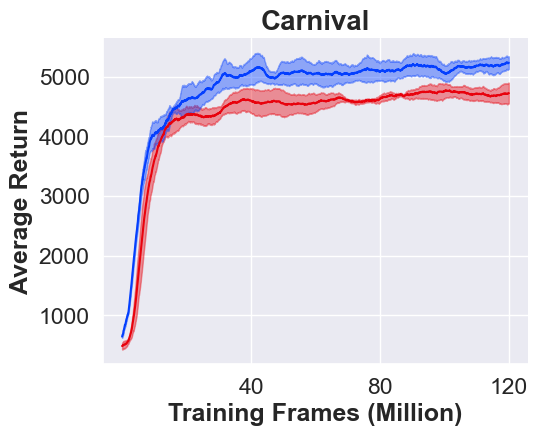} 
\label{fig:4_learning_curves_appendix/CarnivalNoFrameskip-v0_4_learning_curves_appendix.png} 
\end{subfigure}% 
~ 
\begin{subfigure}[t]{ .18\textwidth} 
\centering 
\includegraphics[width=\textwidth]{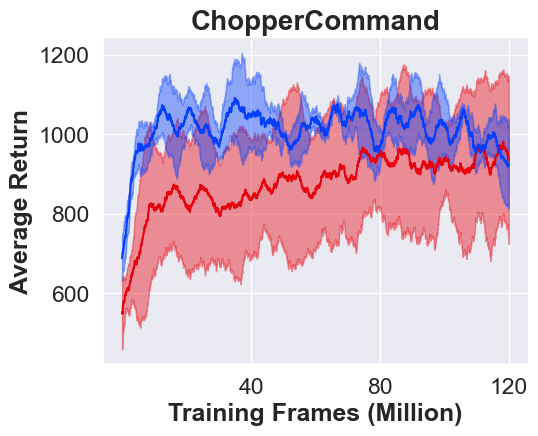} 
\label{fig:4_learning_curves_appendix/ChopperCommandNoFrameskip-v0_4_learning_curves_appendix.png} 
\end{subfigure}% 
~ 
\begin{subfigure}[t]{ .18\textwidth} 
\centering 
\includegraphics[width=\textwidth]{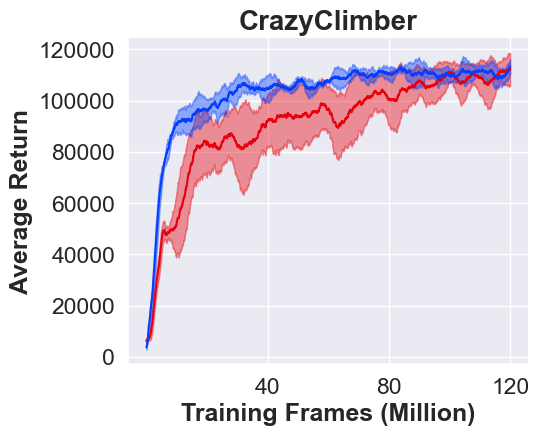} 
\label{fig:4_learning_curves_appendix/CrazyClimberNoFrameskip-v0_4_learning_curves_appendix.png} 
\end{subfigure}% 

\begin{subfigure}[t]{ .18\textwidth} 
\centering 
\includegraphics[width=\textwidth]{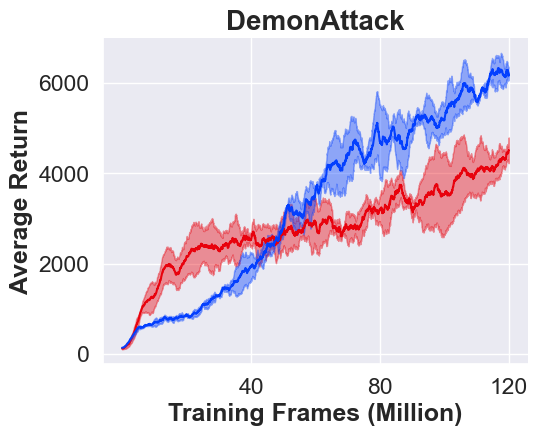} 
\label{fig:4_learning_curves_appendix/DemonAttackNoFrameskip-v0_4_learning_curves_appendix.png} 
\end{subfigure}% 
~ 
\begin{subfigure}[t]{ .18\textwidth} 
\centering 
\includegraphics[width=\textwidth]{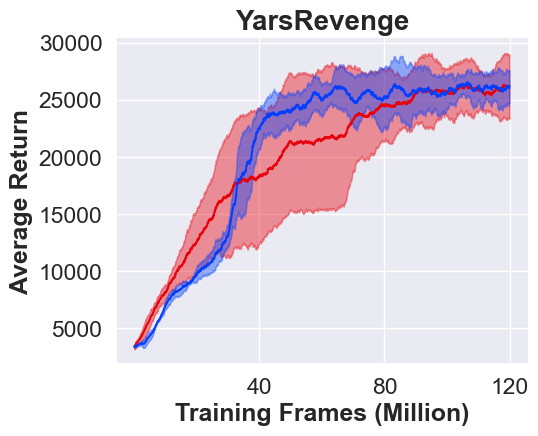} 
\label{fig:4_learning_curves_appendix/YarsRevengeNoFrameskip-v0_4_learning_curves_appendix.png} 
\end{subfigure}% 
~ 
\begin{subfigure}[t]{ .18\textwidth} 
\centering 
\includegraphics[width=\textwidth]{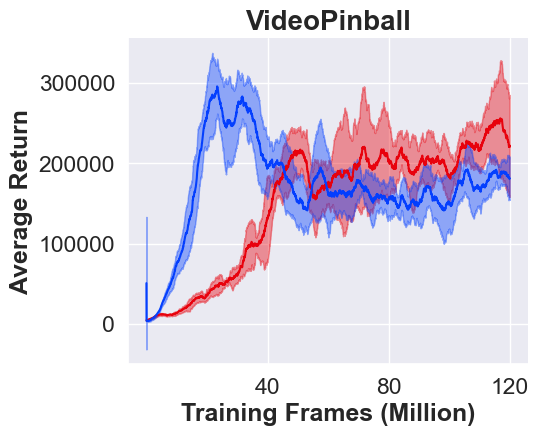} 
\label{fig:4_learning_curves_appendix/VideoPinballNoFrameskip-v0_4_learning_curves_appendix.png} 
\end{subfigure}% 
~ 
\begin{subfigure}[t]{ .18\textwidth} 
\centering 
\includegraphics[width=\textwidth]{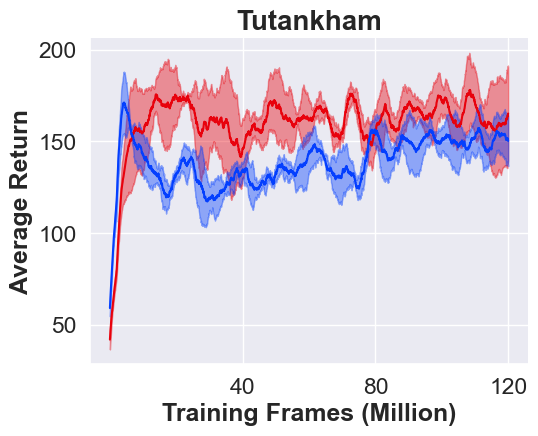} 
\label{fig:4_learning_curves_appendix/TutankhamNoFrameskip-v0_4_learning_curves_appendix.png} 
\end{subfigure}% 
~ 
\begin{subfigure}[t]{ .18\textwidth} 
\centering 
\includegraphics[width=\textwidth]{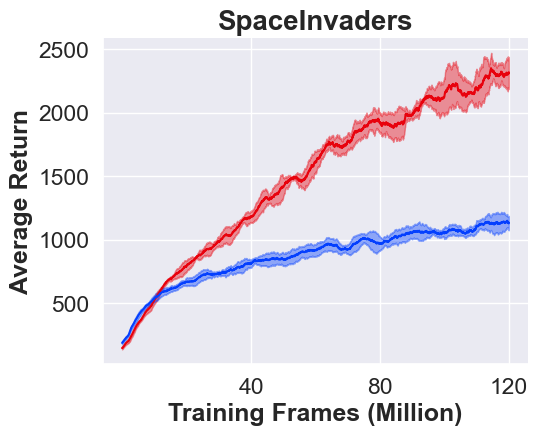} 
\label{fig:4_learning_curves_appendix/SpaceInvadersNoFrameskip-v0_4_learning_curves_appendix.png} 
\end{subfigure}% 

\begin{subfigure}[t]{ .18\textwidth} 
\centering 
\includegraphics[width=\textwidth]{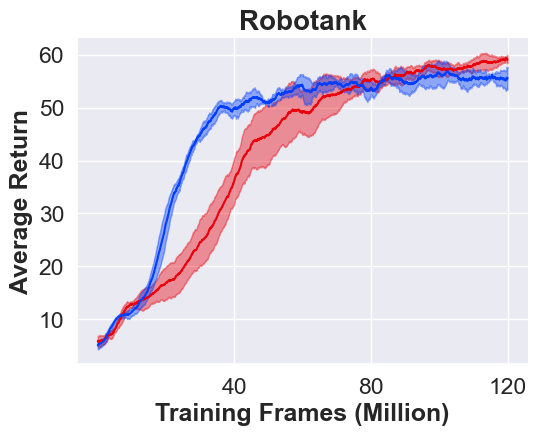} 
\label{fig:4_learning_curves_appendix/RobotankNoFrameskip-v0_4_learning_curves_appendix.png} 
\end{subfigure}% 
~ 
\begin{subfigure}[t]{ .18\textwidth} 
\centering 
\includegraphics[width=\textwidth]{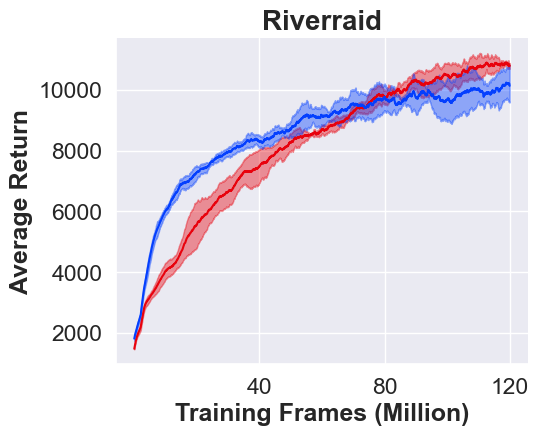} 
\label{fig:4_learning_curves_appendix/RiverraidNoFrameskip-v0_4_learning_curves_appendix.png} 
\end{subfigure}% 
~ 
\begin{subfigure}[t]{ .18\textwidth} 
\centering 
\includegraphics[width=\textwidth]{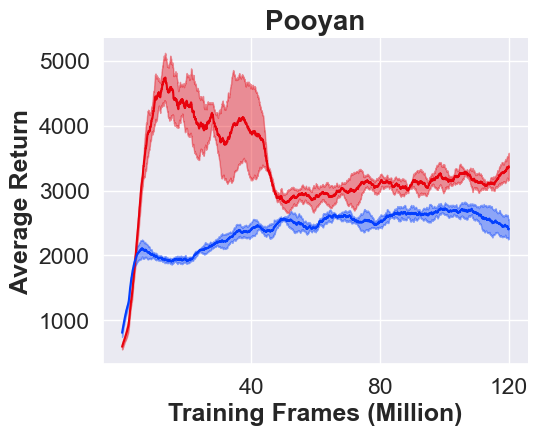} 
\label{fig:4_learning_curves_appendix/PooyanNoFrameskip-v0_4_learning_curves_appendix.png} 
\end{subfigure}% 
~ 
\begin{subfigure}[t]{ .18\textwidth} 
\centering 
\includegraphics[width=\textwidth]{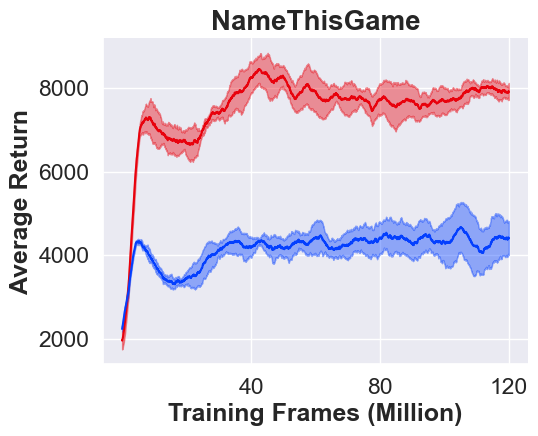} 
\label{fig:4_learning_curves_appendix/NameThisGameNoFrameskip-v0_4_learning_curves_appendix.png} 
\end{subfigure}% 
~ 
\begin{subfigure}[t]{ .18\textwidth} 
\centering 
\includegraphics[width=\textwidth]{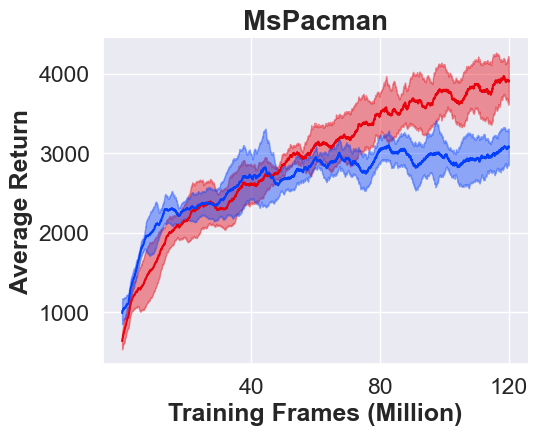} 
\label{fig:4_learning_curves_appendix/MsPacmanNoFrameskip-v0_4_learning_curves_appendix.png} 
\end{subfigure}% 

\begin{subfigure}[t]{ .18\textwidth} 
\centering 
\includegraphics[width=\textwidth]{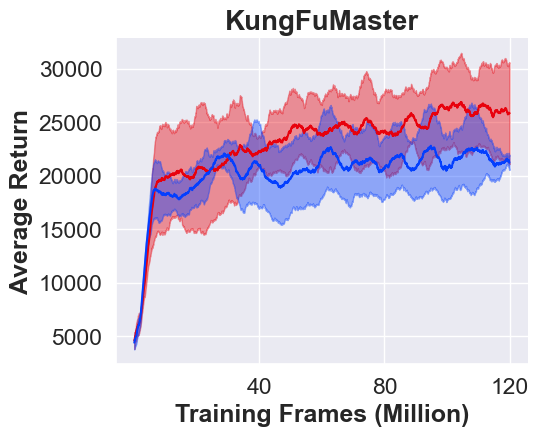} 
\label{fig:4_learning_curves_appendix/KungFuMasterNoFrameskip-v0_4_learning_curves_appendix.png} 
\end{subfigure}% 
~ 
\begin{subfigure}[t]{ .18\textwidth} 
\centering 
\includegraphics[width=\textwidth]{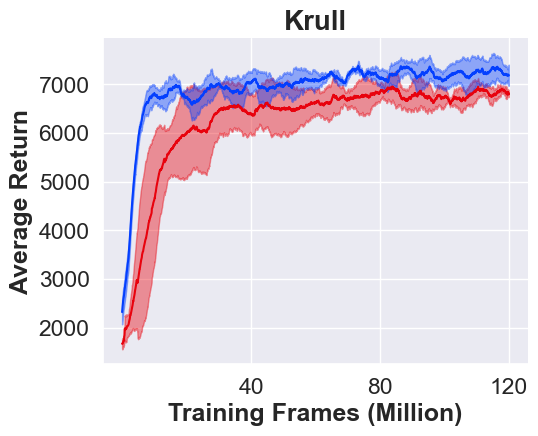} 
\label{fig:4_learning_curves_appendix/KrullNoFrameskip-v0_4_learning_curves_appendix.png} 
\end{subfigure}% 
~ 
\begin{subfigure}[t]{ .18\textwidth} 
\centering 
\includegraphics[width=\textwidth]{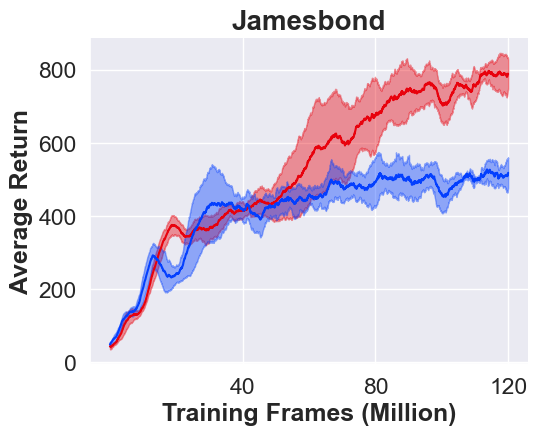} 
\label{fig:4_learning_curves_appendix/JamesbondNoFrameskip-v0_4_learning_curves_appendix.png} 
\end{subfigure}% 
~ 
\begin{subfigure}[t]{ .18\textwidth} 
\centering 
\includegraphics[width=\textwidth]{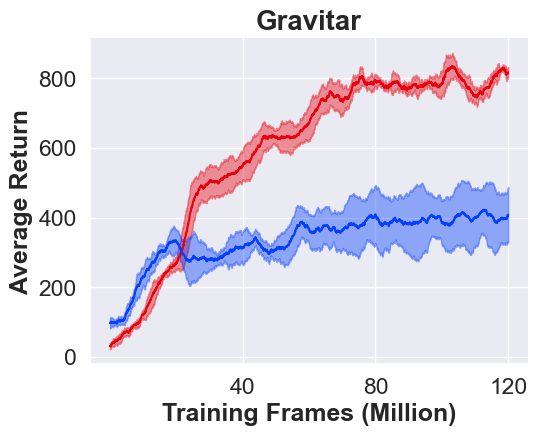} 
\label{fig:4_learning_curves_appendix/GravitarNoFrameskip-v0_4_learning_curves_appendix.png} 
\end{subfigure}% 
~ 
\begin{subfigure}[t]{ .18\textwidth} 
\centering 
\includegraphics[width=\textwidth]{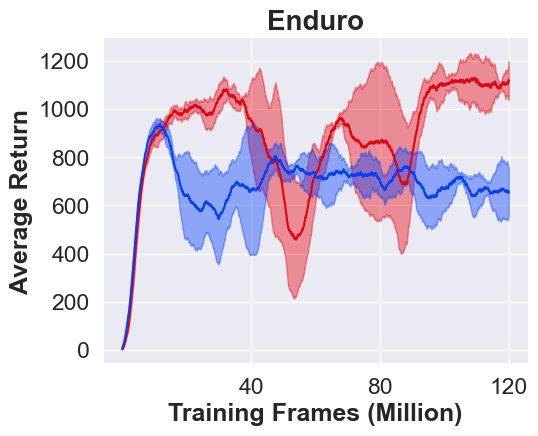} 
\label{fig:4_learning_curves_appendix/EnduroNoFrameskip-v0_4_learning_curves_appendix.png} 
\end{subfigure}% 

\caption{\textbf{Learning curves for DQN (blue) and \algname{} (red)} on 40 Atari games. X-axis indicates the number of steps from the environment used in training and Y-axis shows average undiscounted return}
\label{fig:main} 
\end{figure} 
\input{rebut}

\clearpage
\bibliographysi{reference}
\bibliographystylesi{abbrvnat}
